# Supplementary material for: Stochastic optimization in digital pre-distortion of the signal
Source: arXiv:2201.12159 source file (2022-01-28)
Supplement: Supplementary file 1 [file appendix.tex]

\begin{figure}[H]
    \centering
     \subfloat[${L_1}$ в оптимизаторе Adam]{{\includegraphics[width=0.45\textwidth]{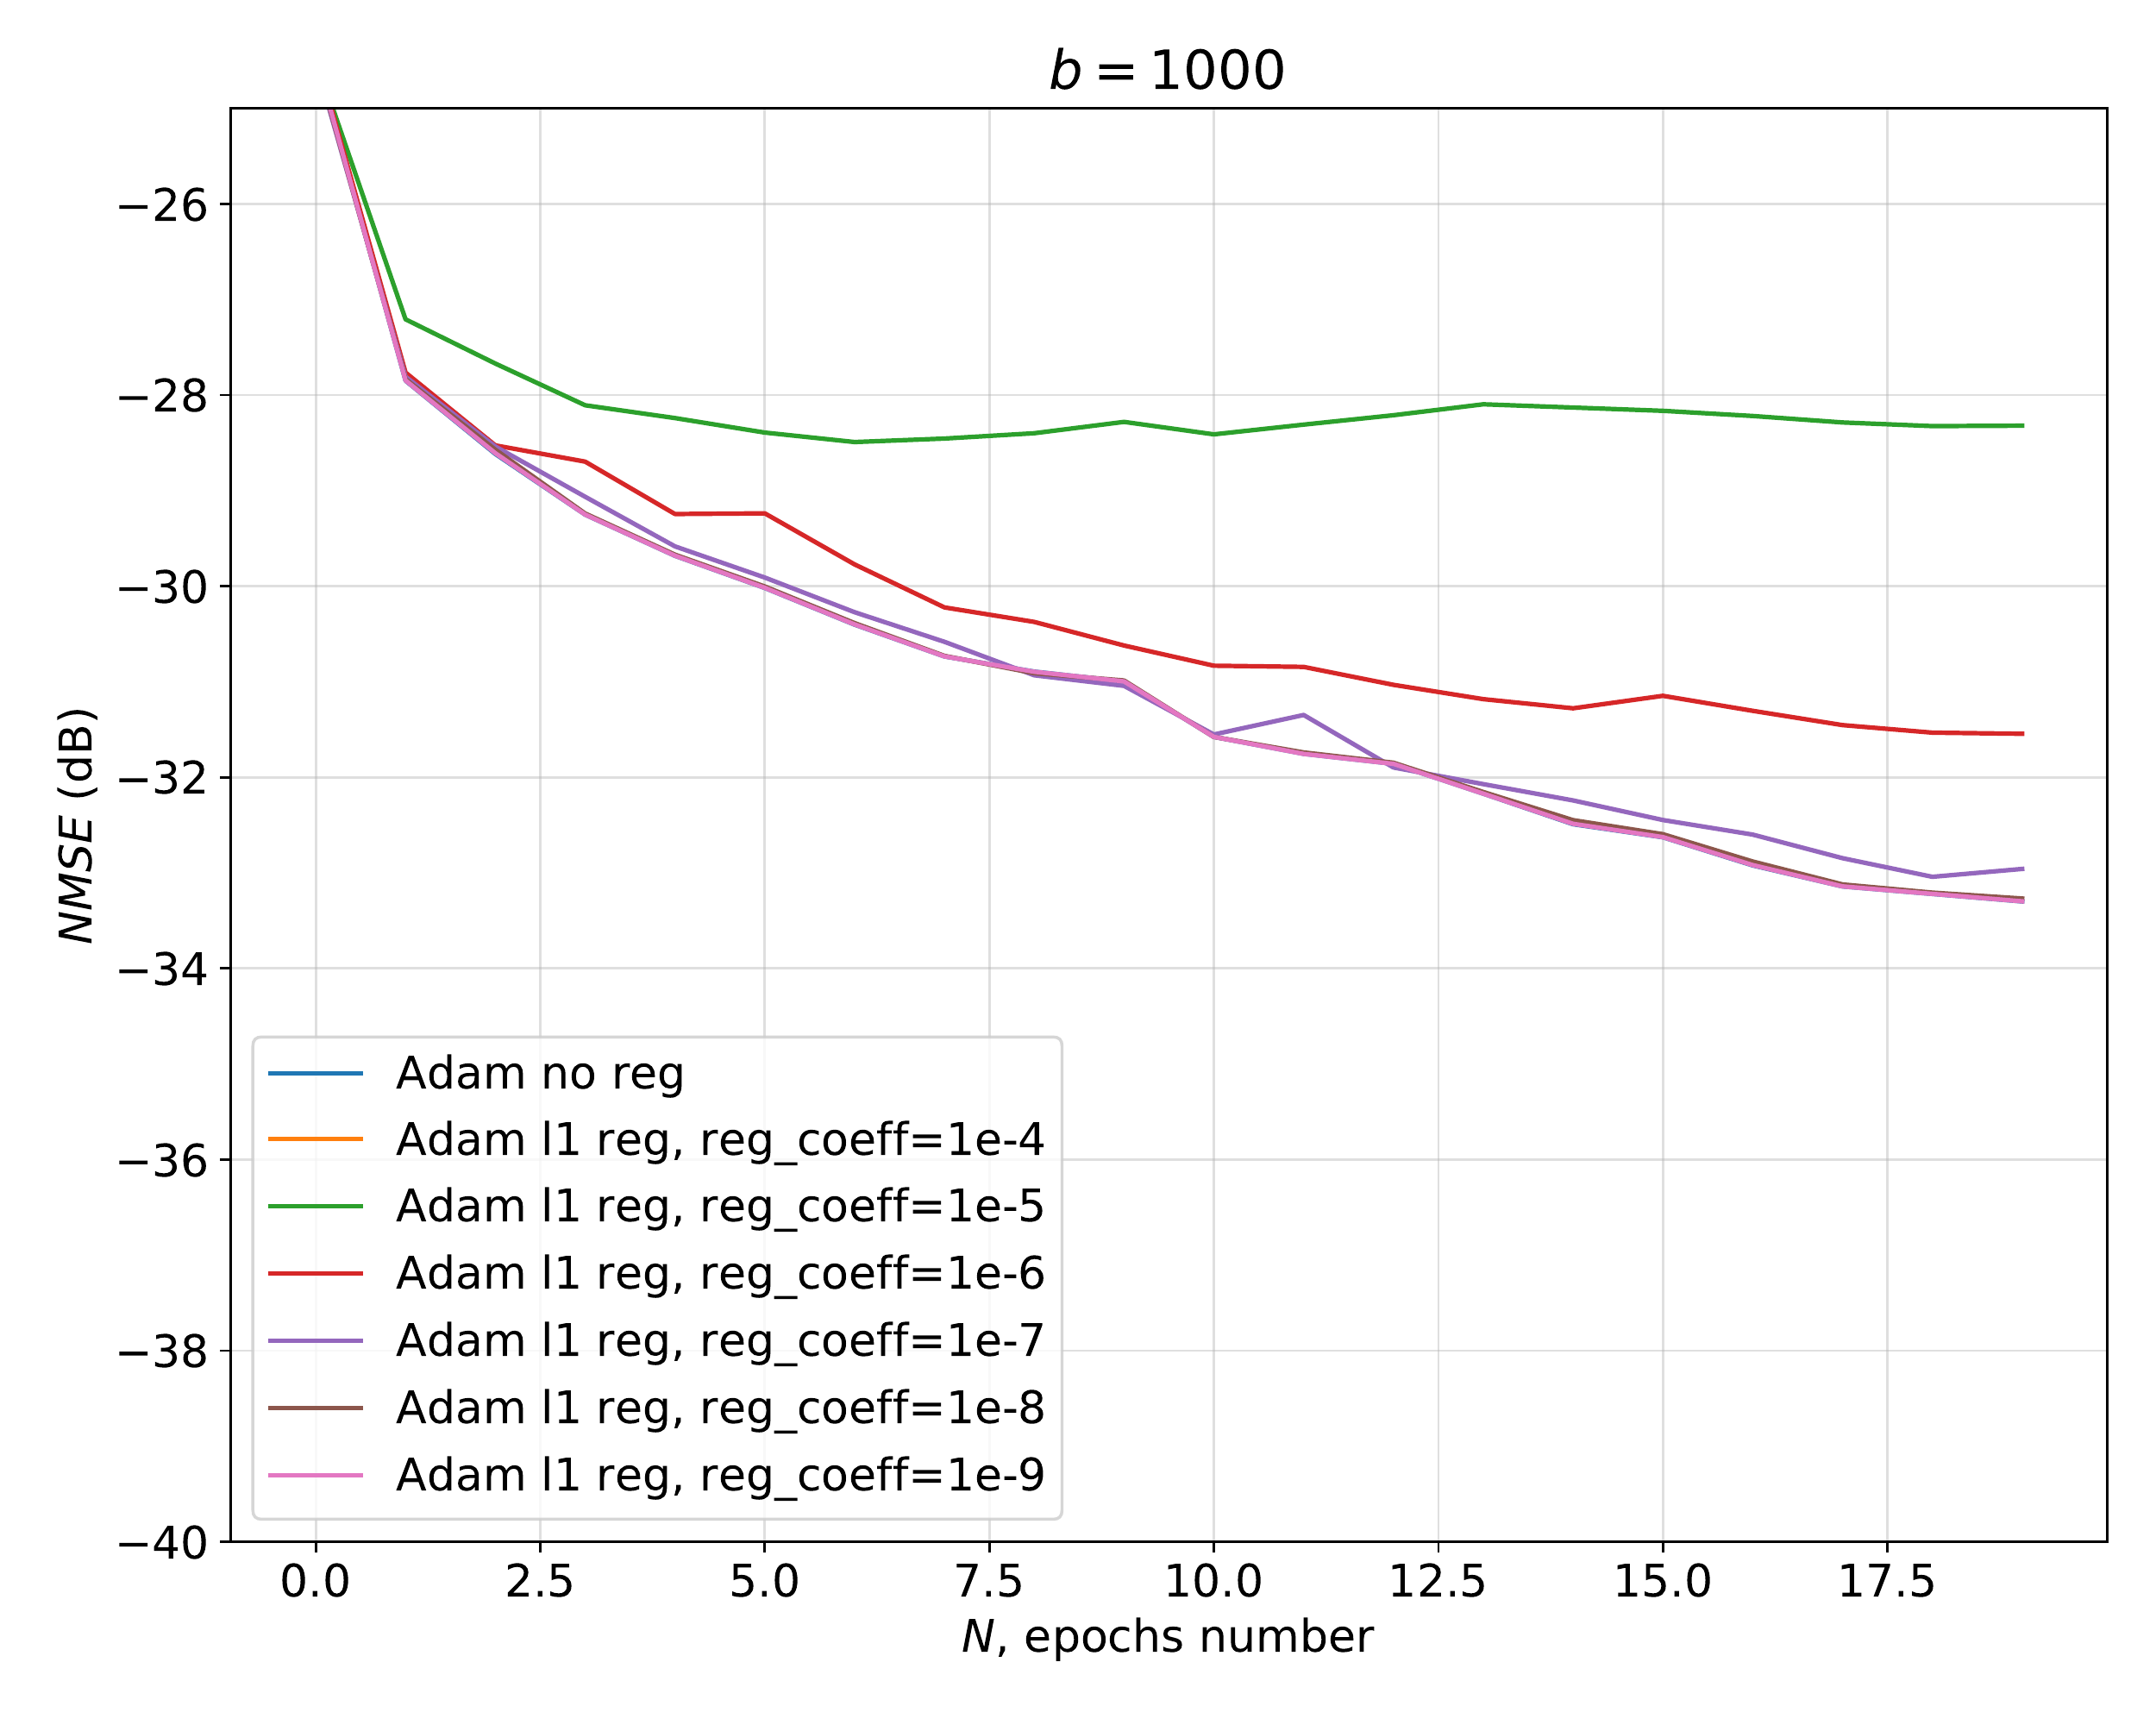}}}
     \subfloat[${L_1}$ в оптимизаторе RAdam]{{\includegraphics[width=0.45\textwidth]{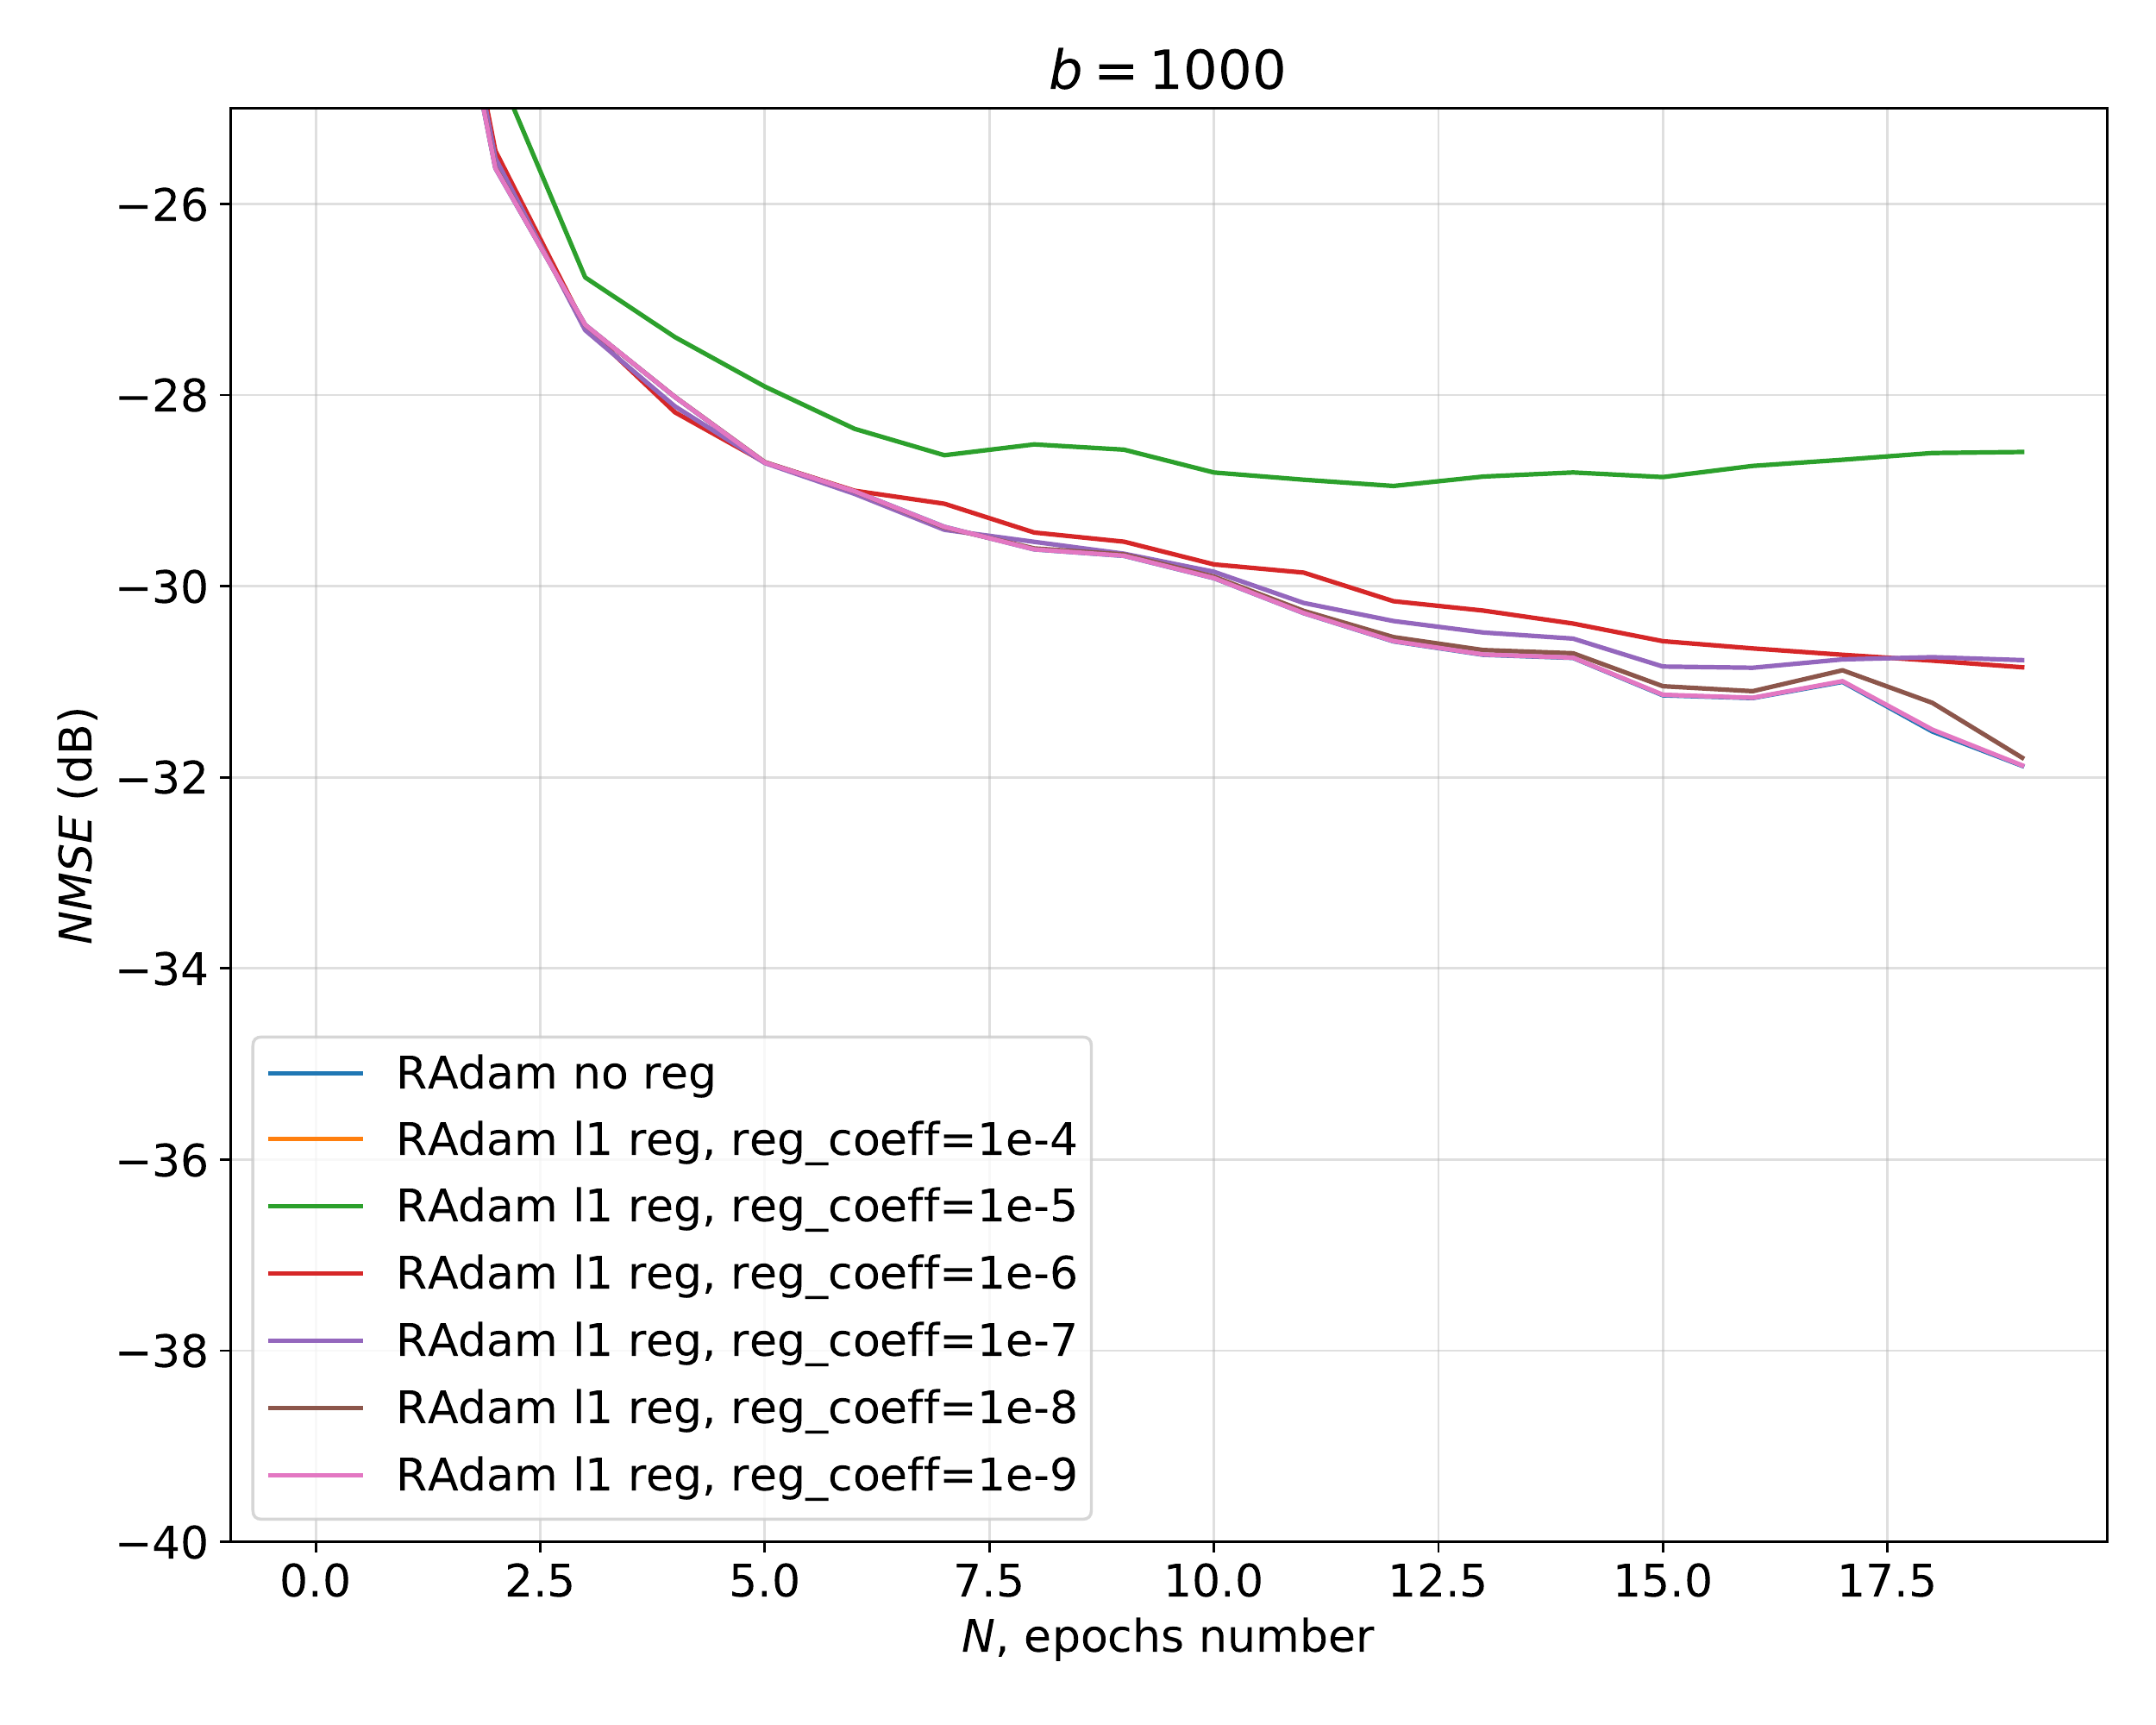}}}

\end{figure}
\begin{figure}[H]
    \centering
     \subfloat[${L_2}$ в оптимизаторе Adam]{{\includegraphics[width=0.45\textwidth]{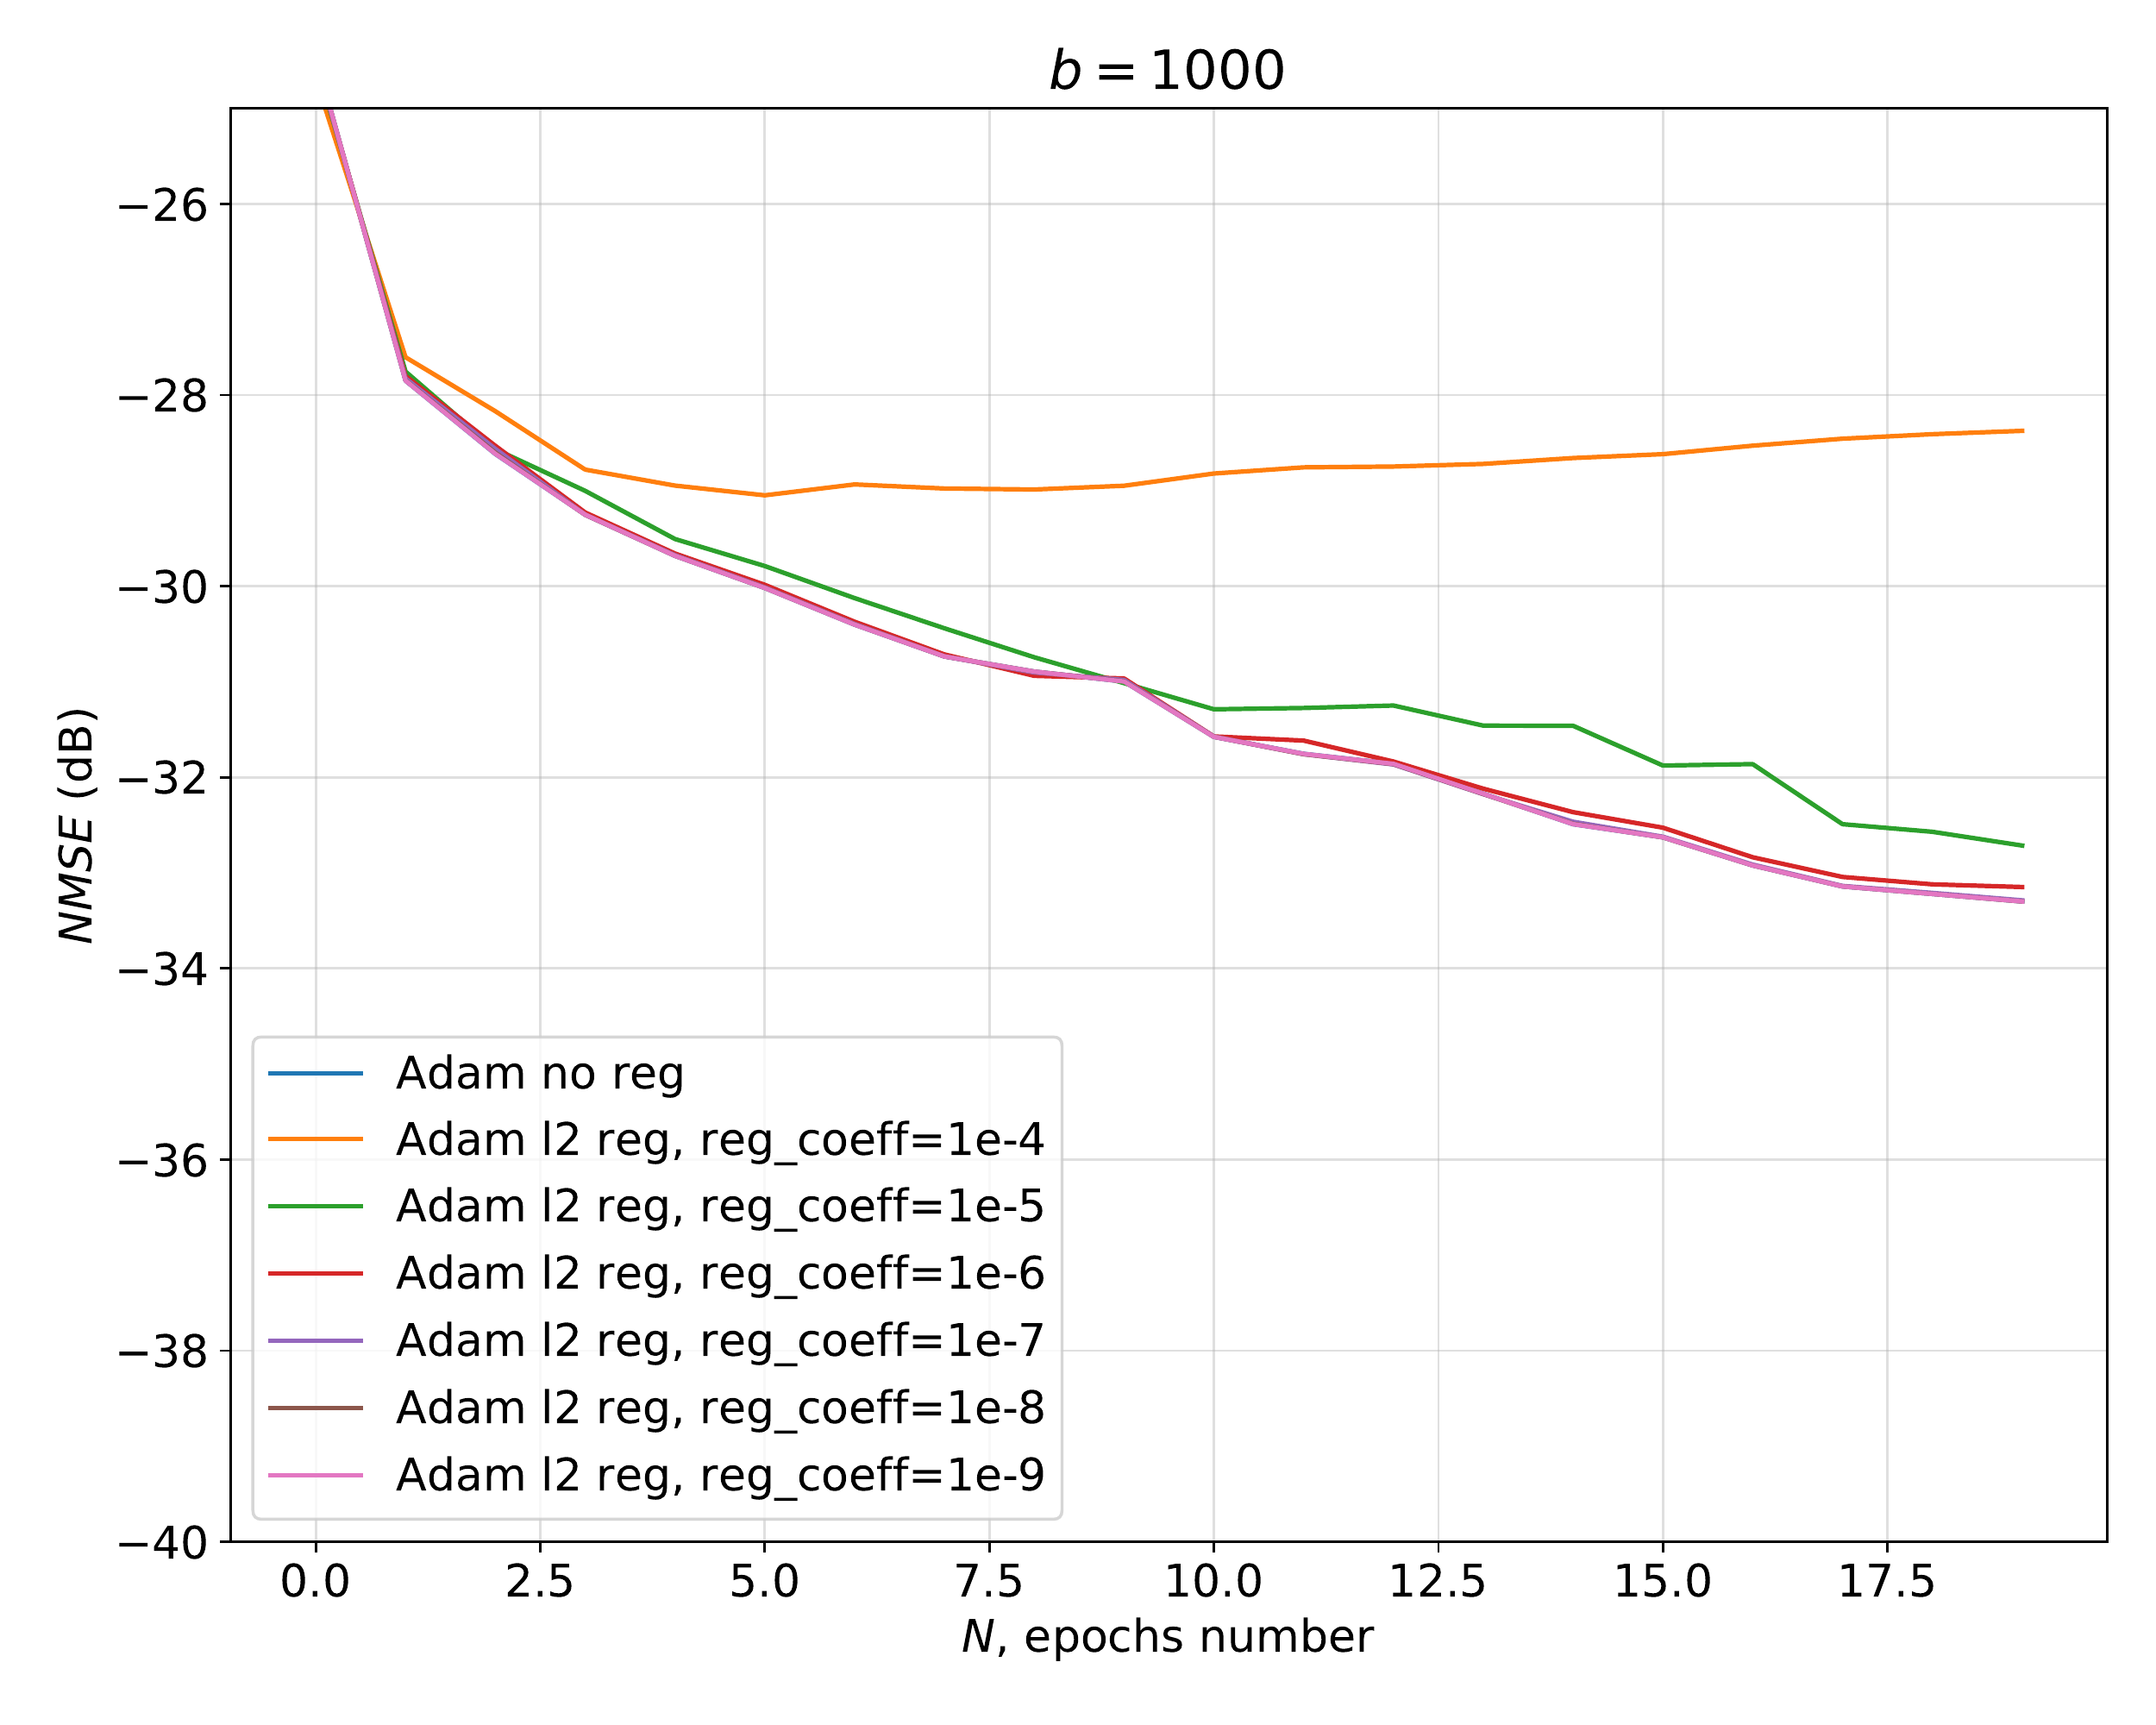}}}
     \subfloat[${L_2}$ в оптимизаторе RAdam]{{\includegraphics[width=0.45\textwidth]{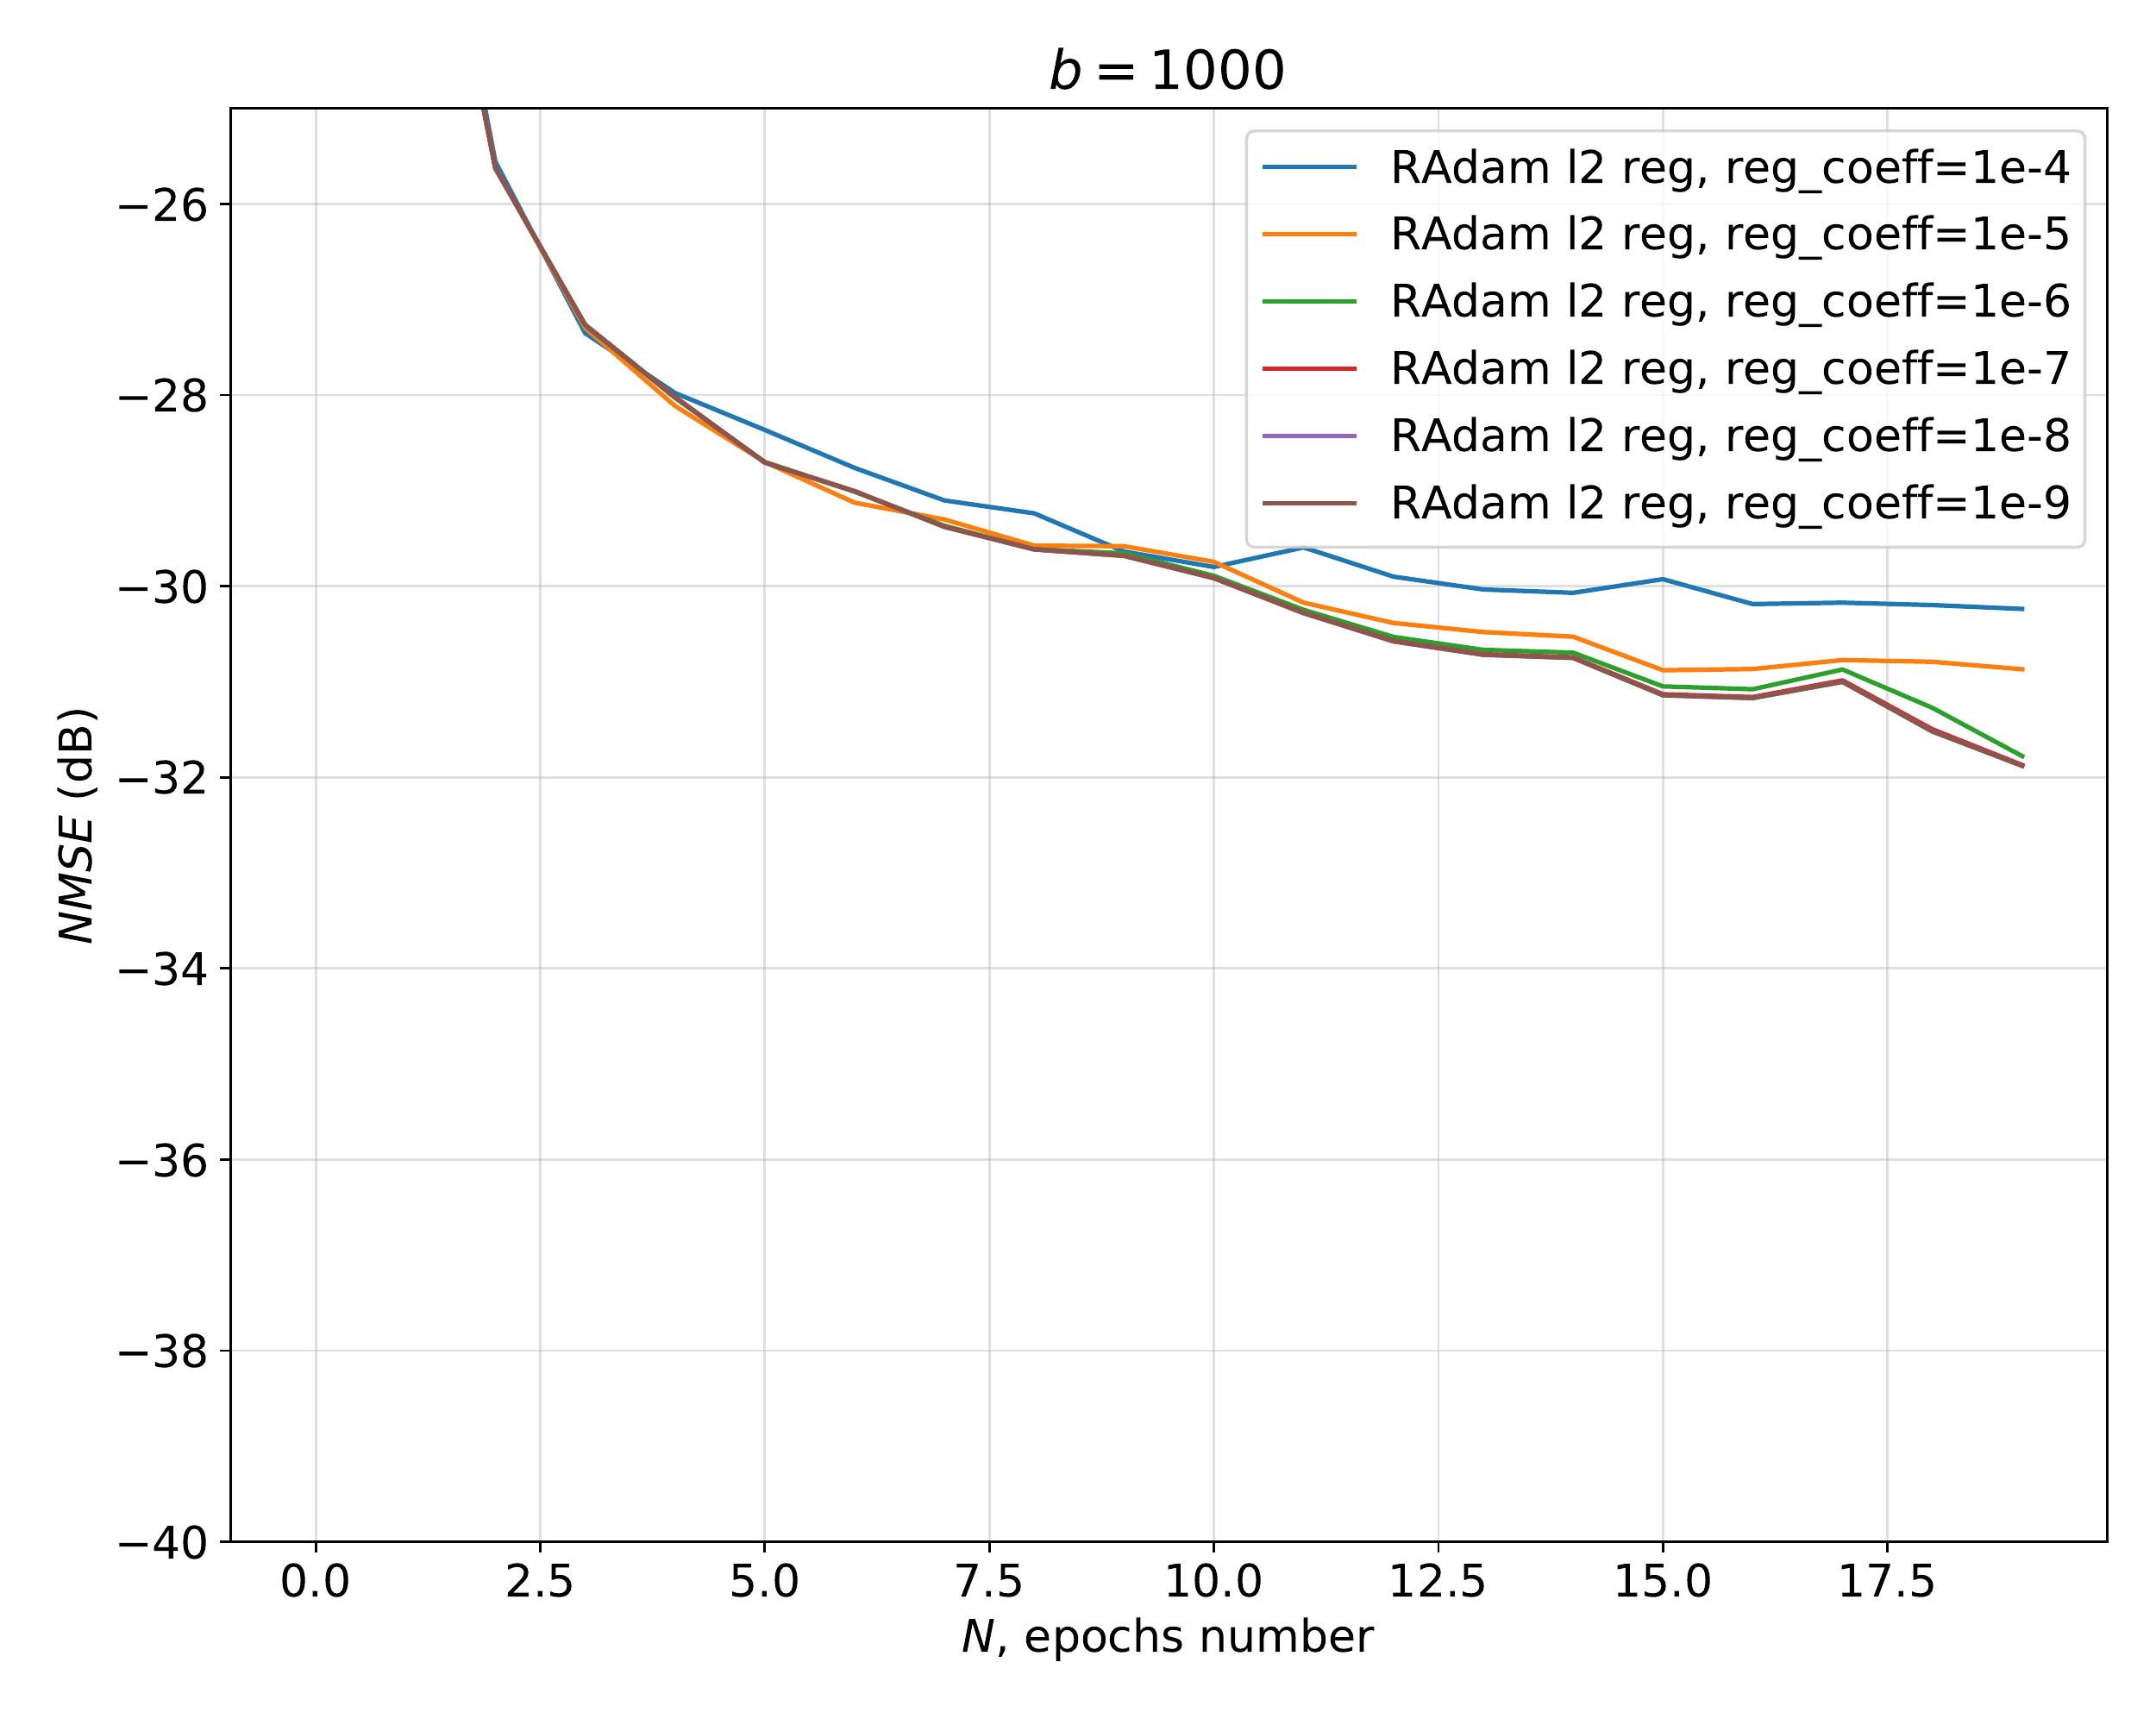}}}

\end{figure}

\begin{figure}[H]
    \centering
    \subfloat[${L_1}$ в оптимизаторе Adam]{{\includegraphics[width=0.45\textwidth]{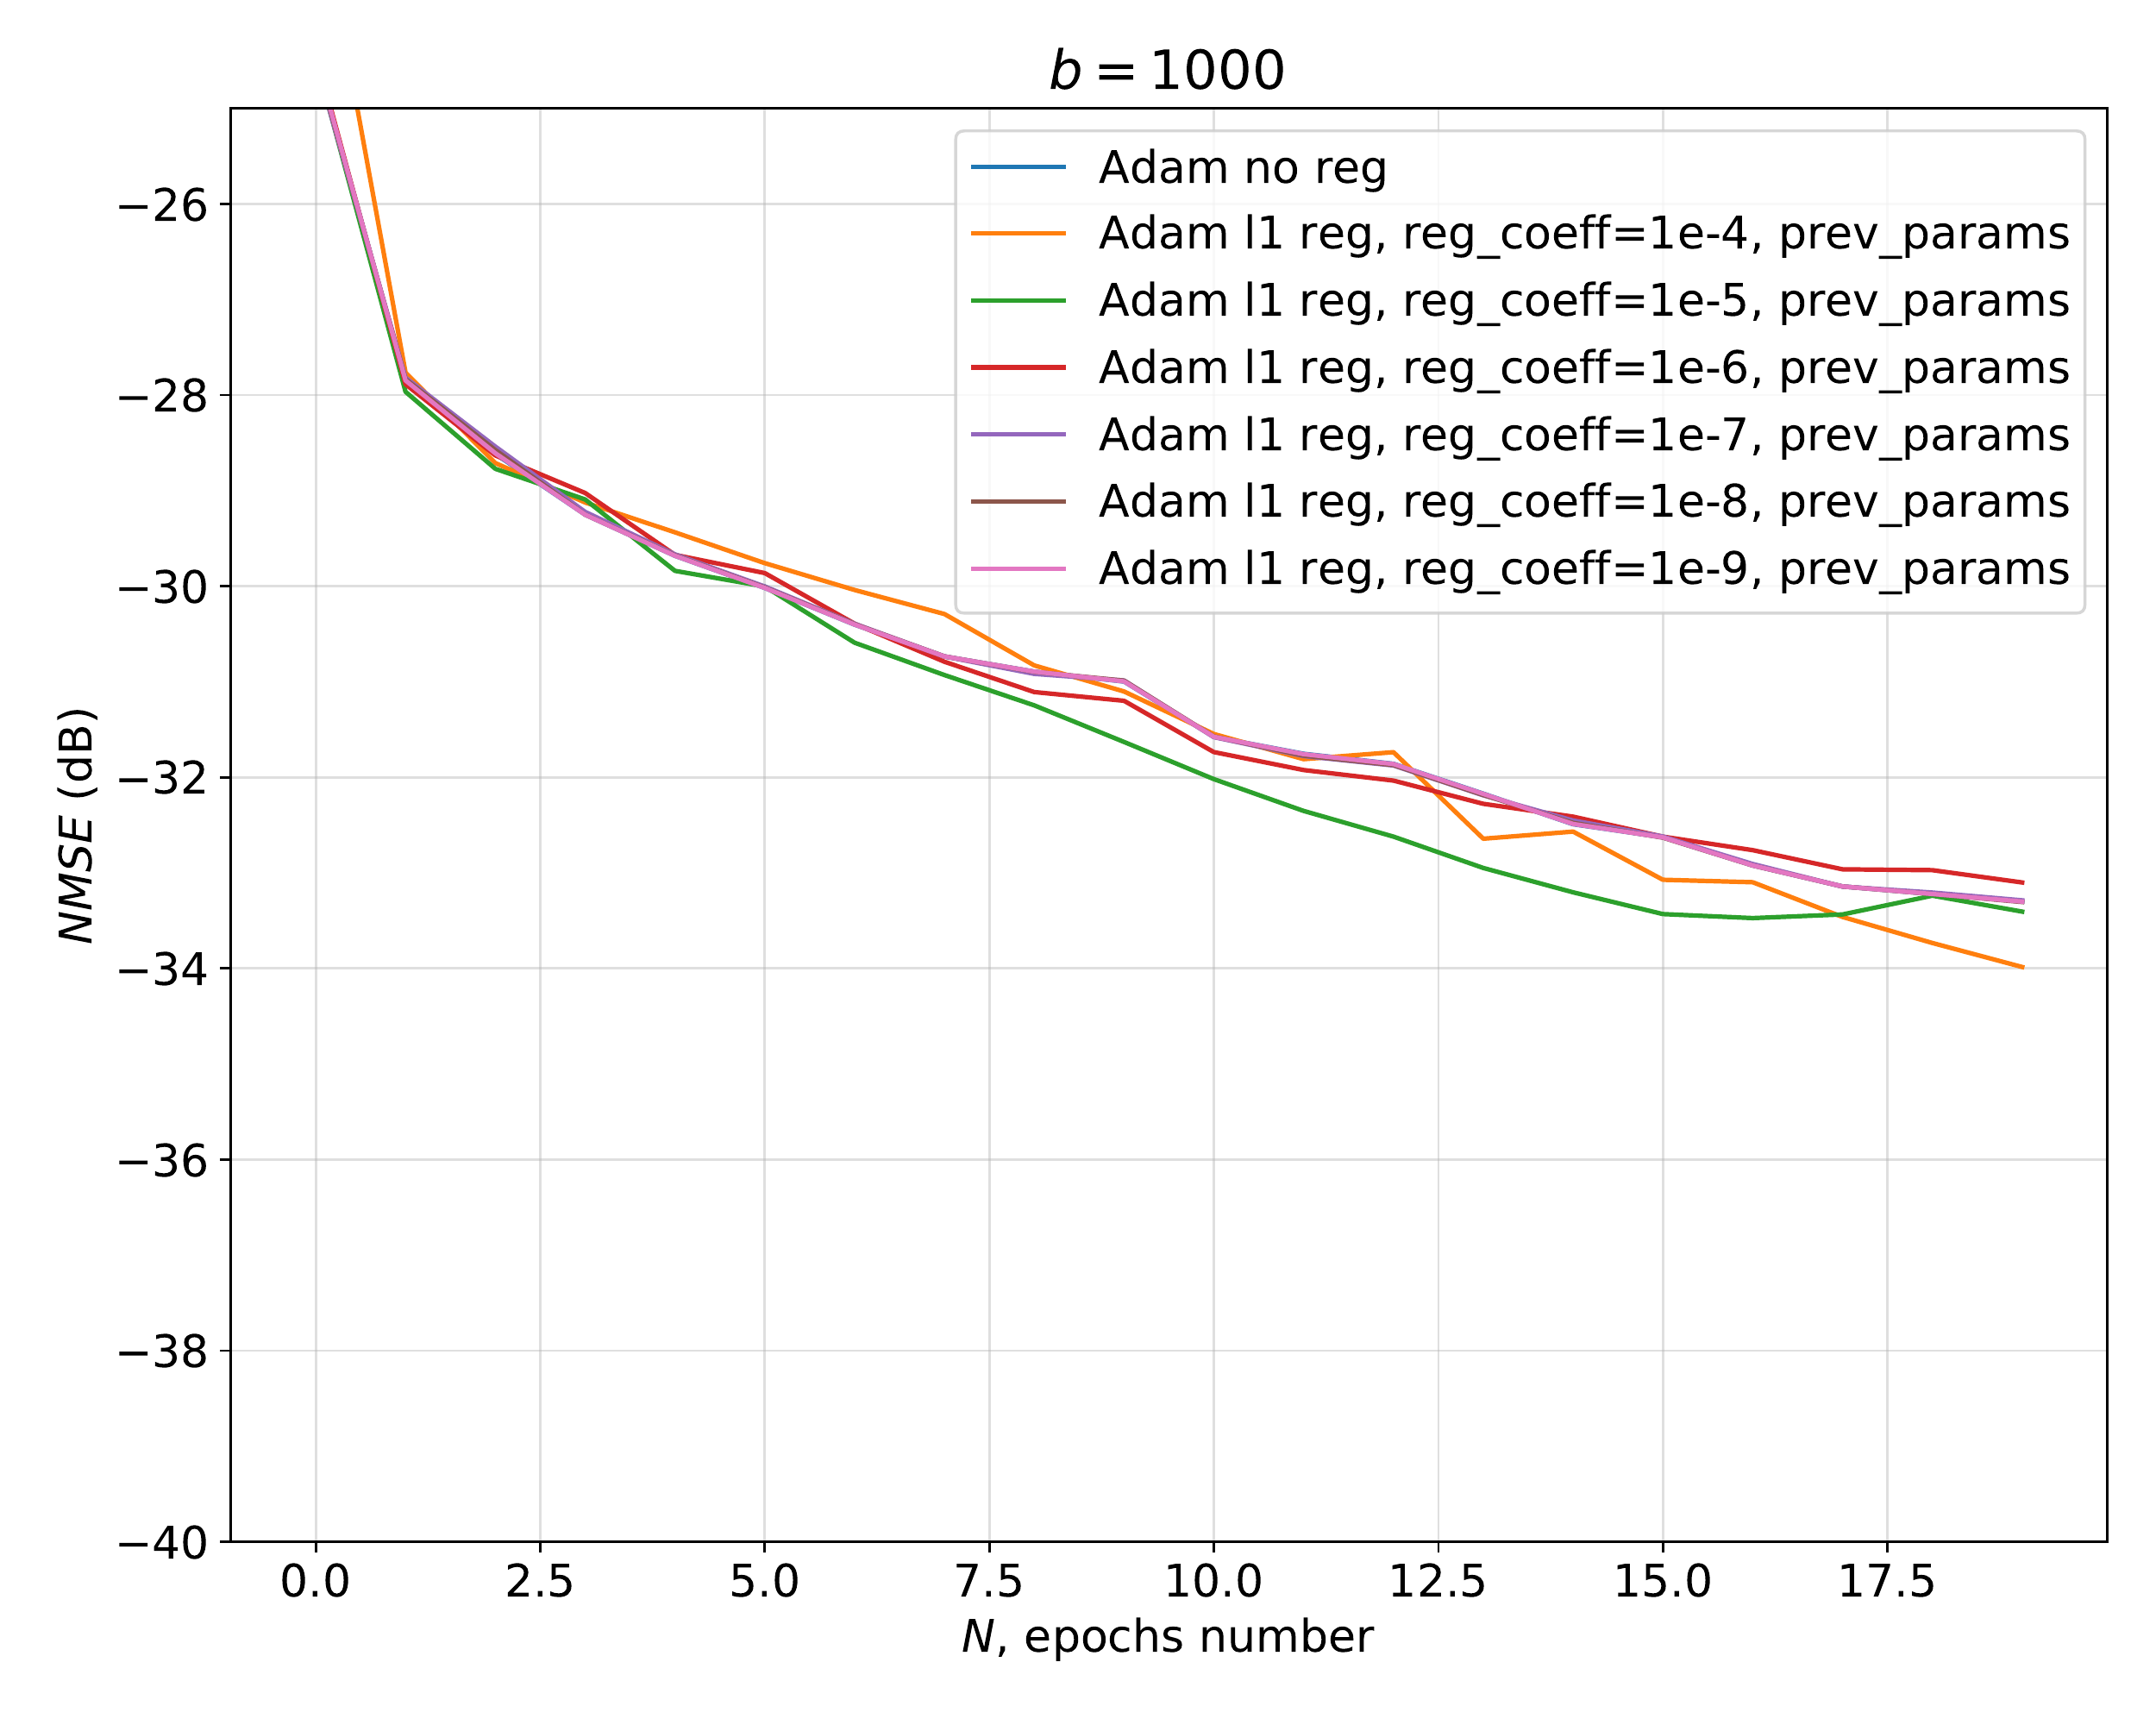}}}
    \subfloat[${L_1}$ в оптимизаторе RAdam]{{\includegraphics[width=0.45\textwidth]{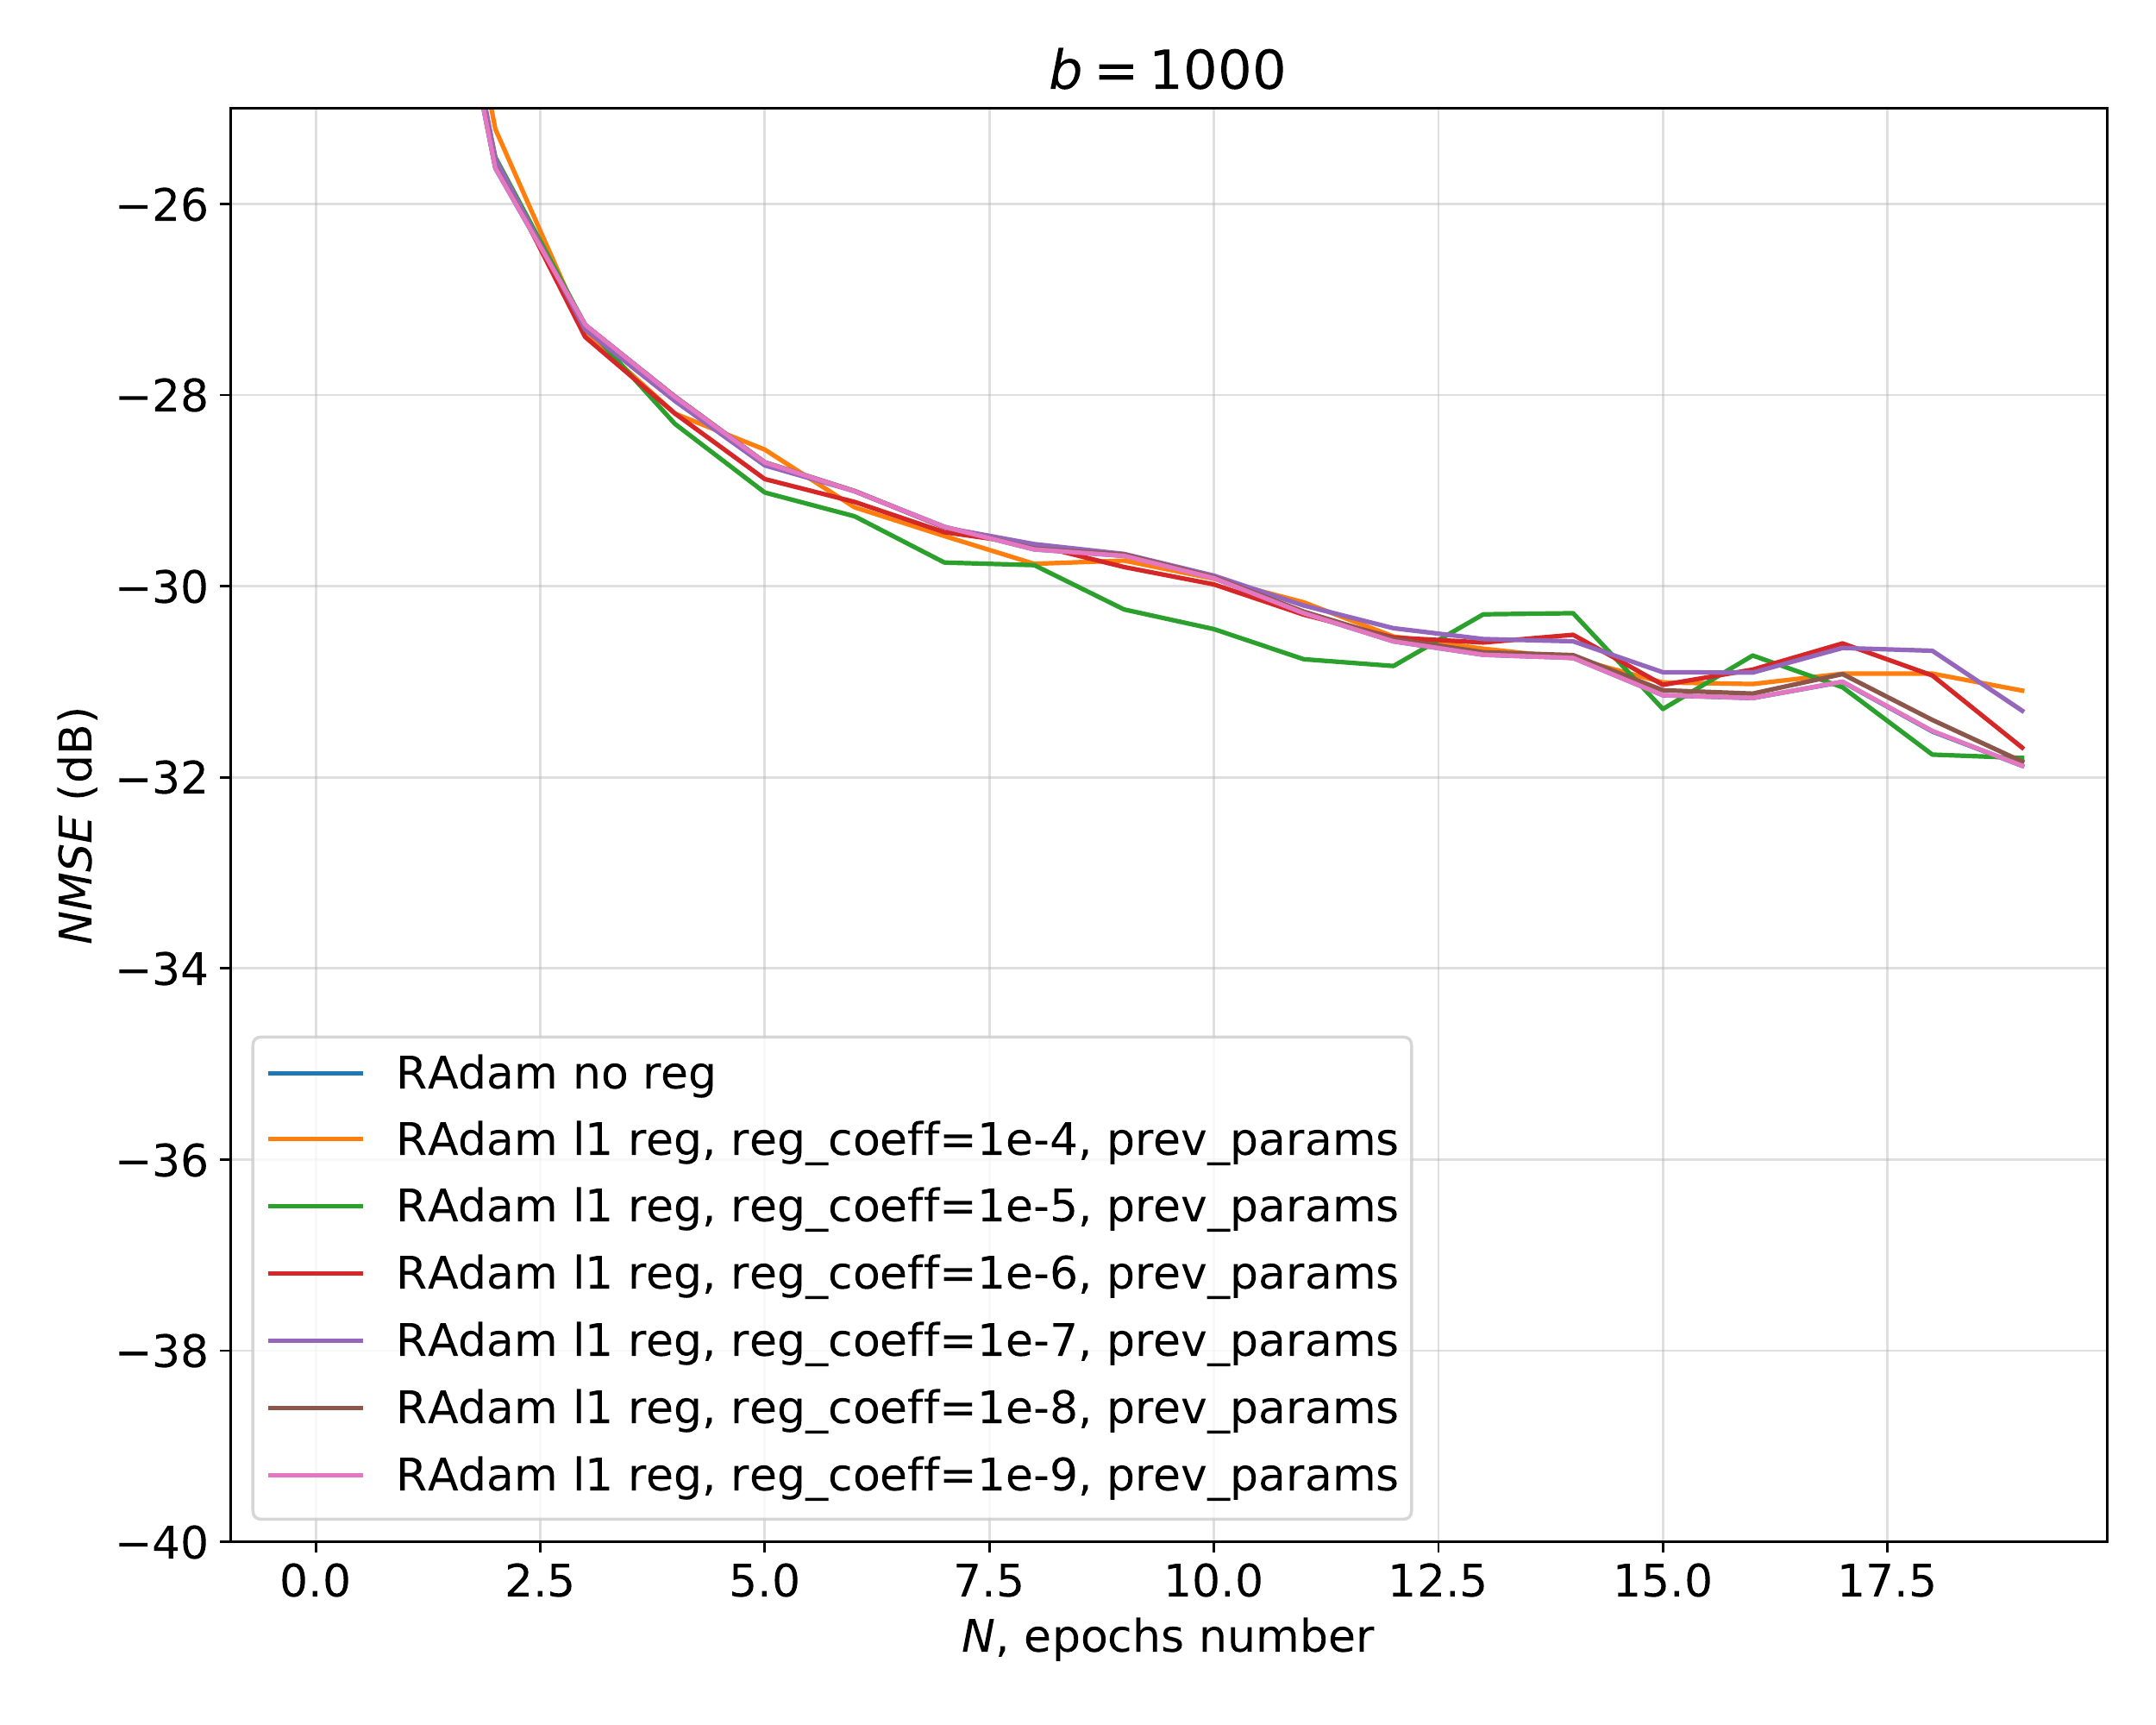}}}

\end{figure}
\begin{figure}[H]
    \centering
    \subfloat[${L_2}$ в оптимизаторе Adam]{{\includegraphics[width=0.45\textwidth]{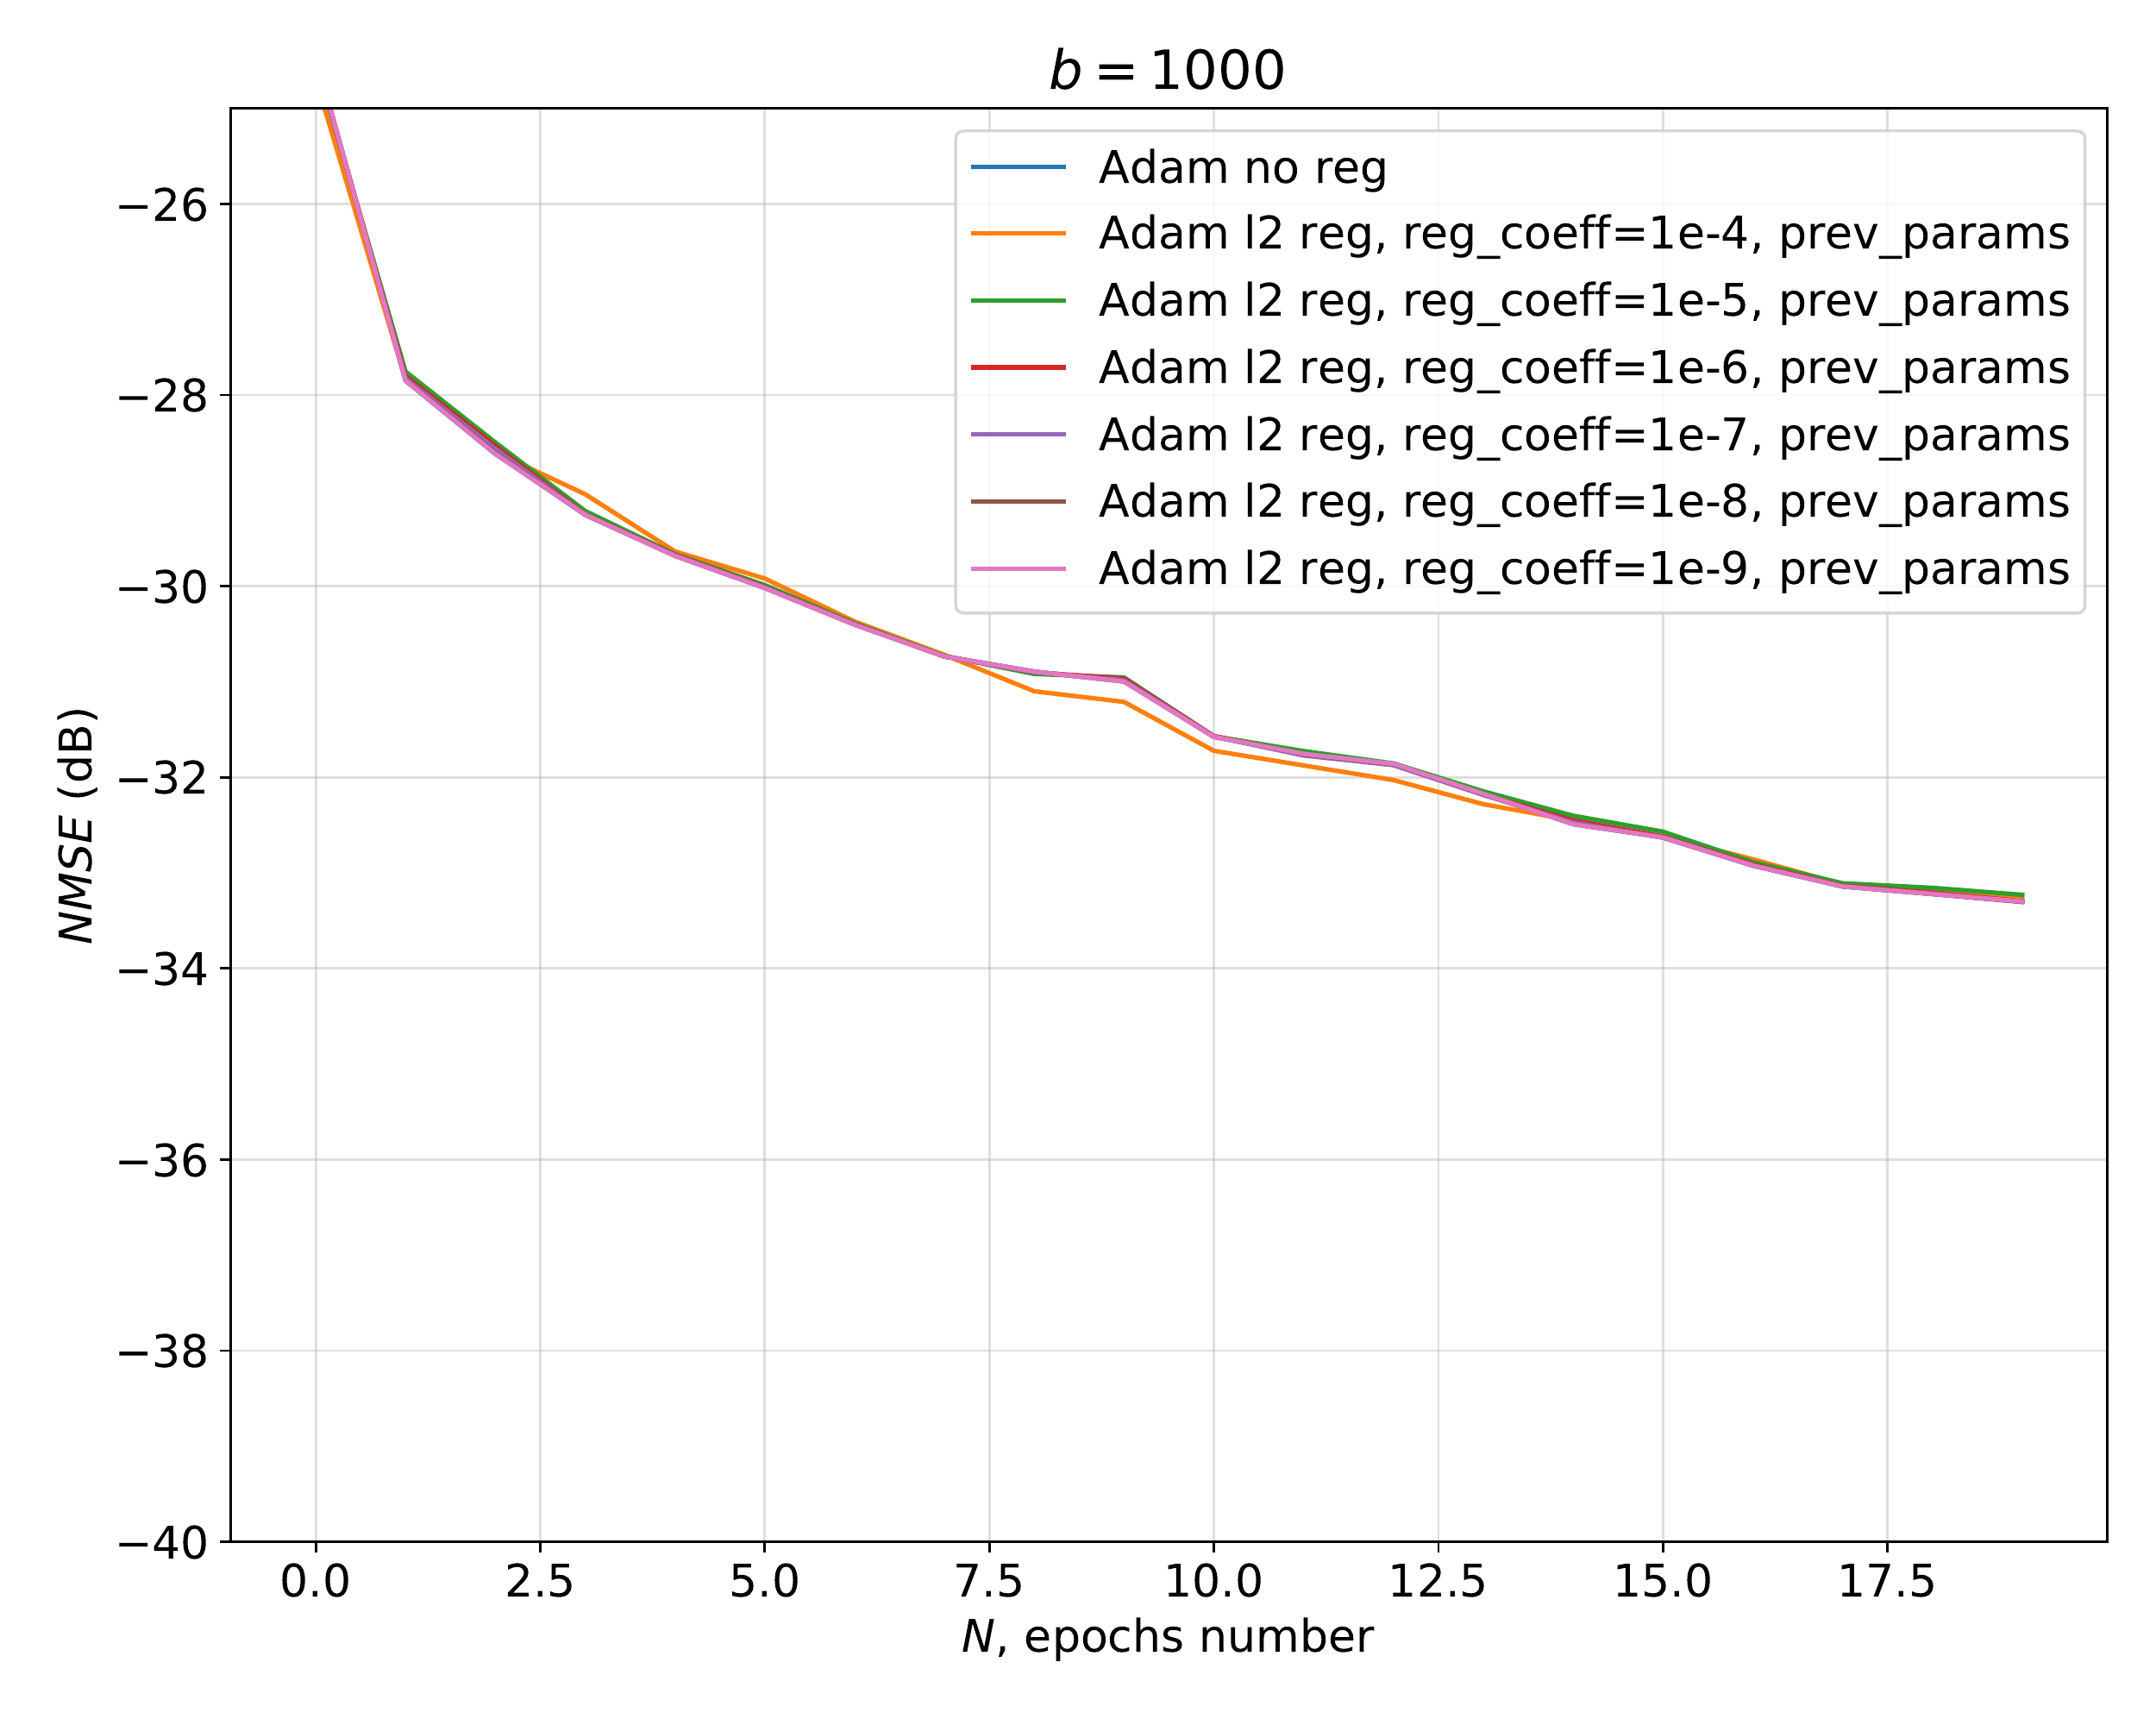}}}
    \subfloat[${L_2}$ в оптимизаторе RAdam]{{\includegraphics[width=0.45\textwidth]{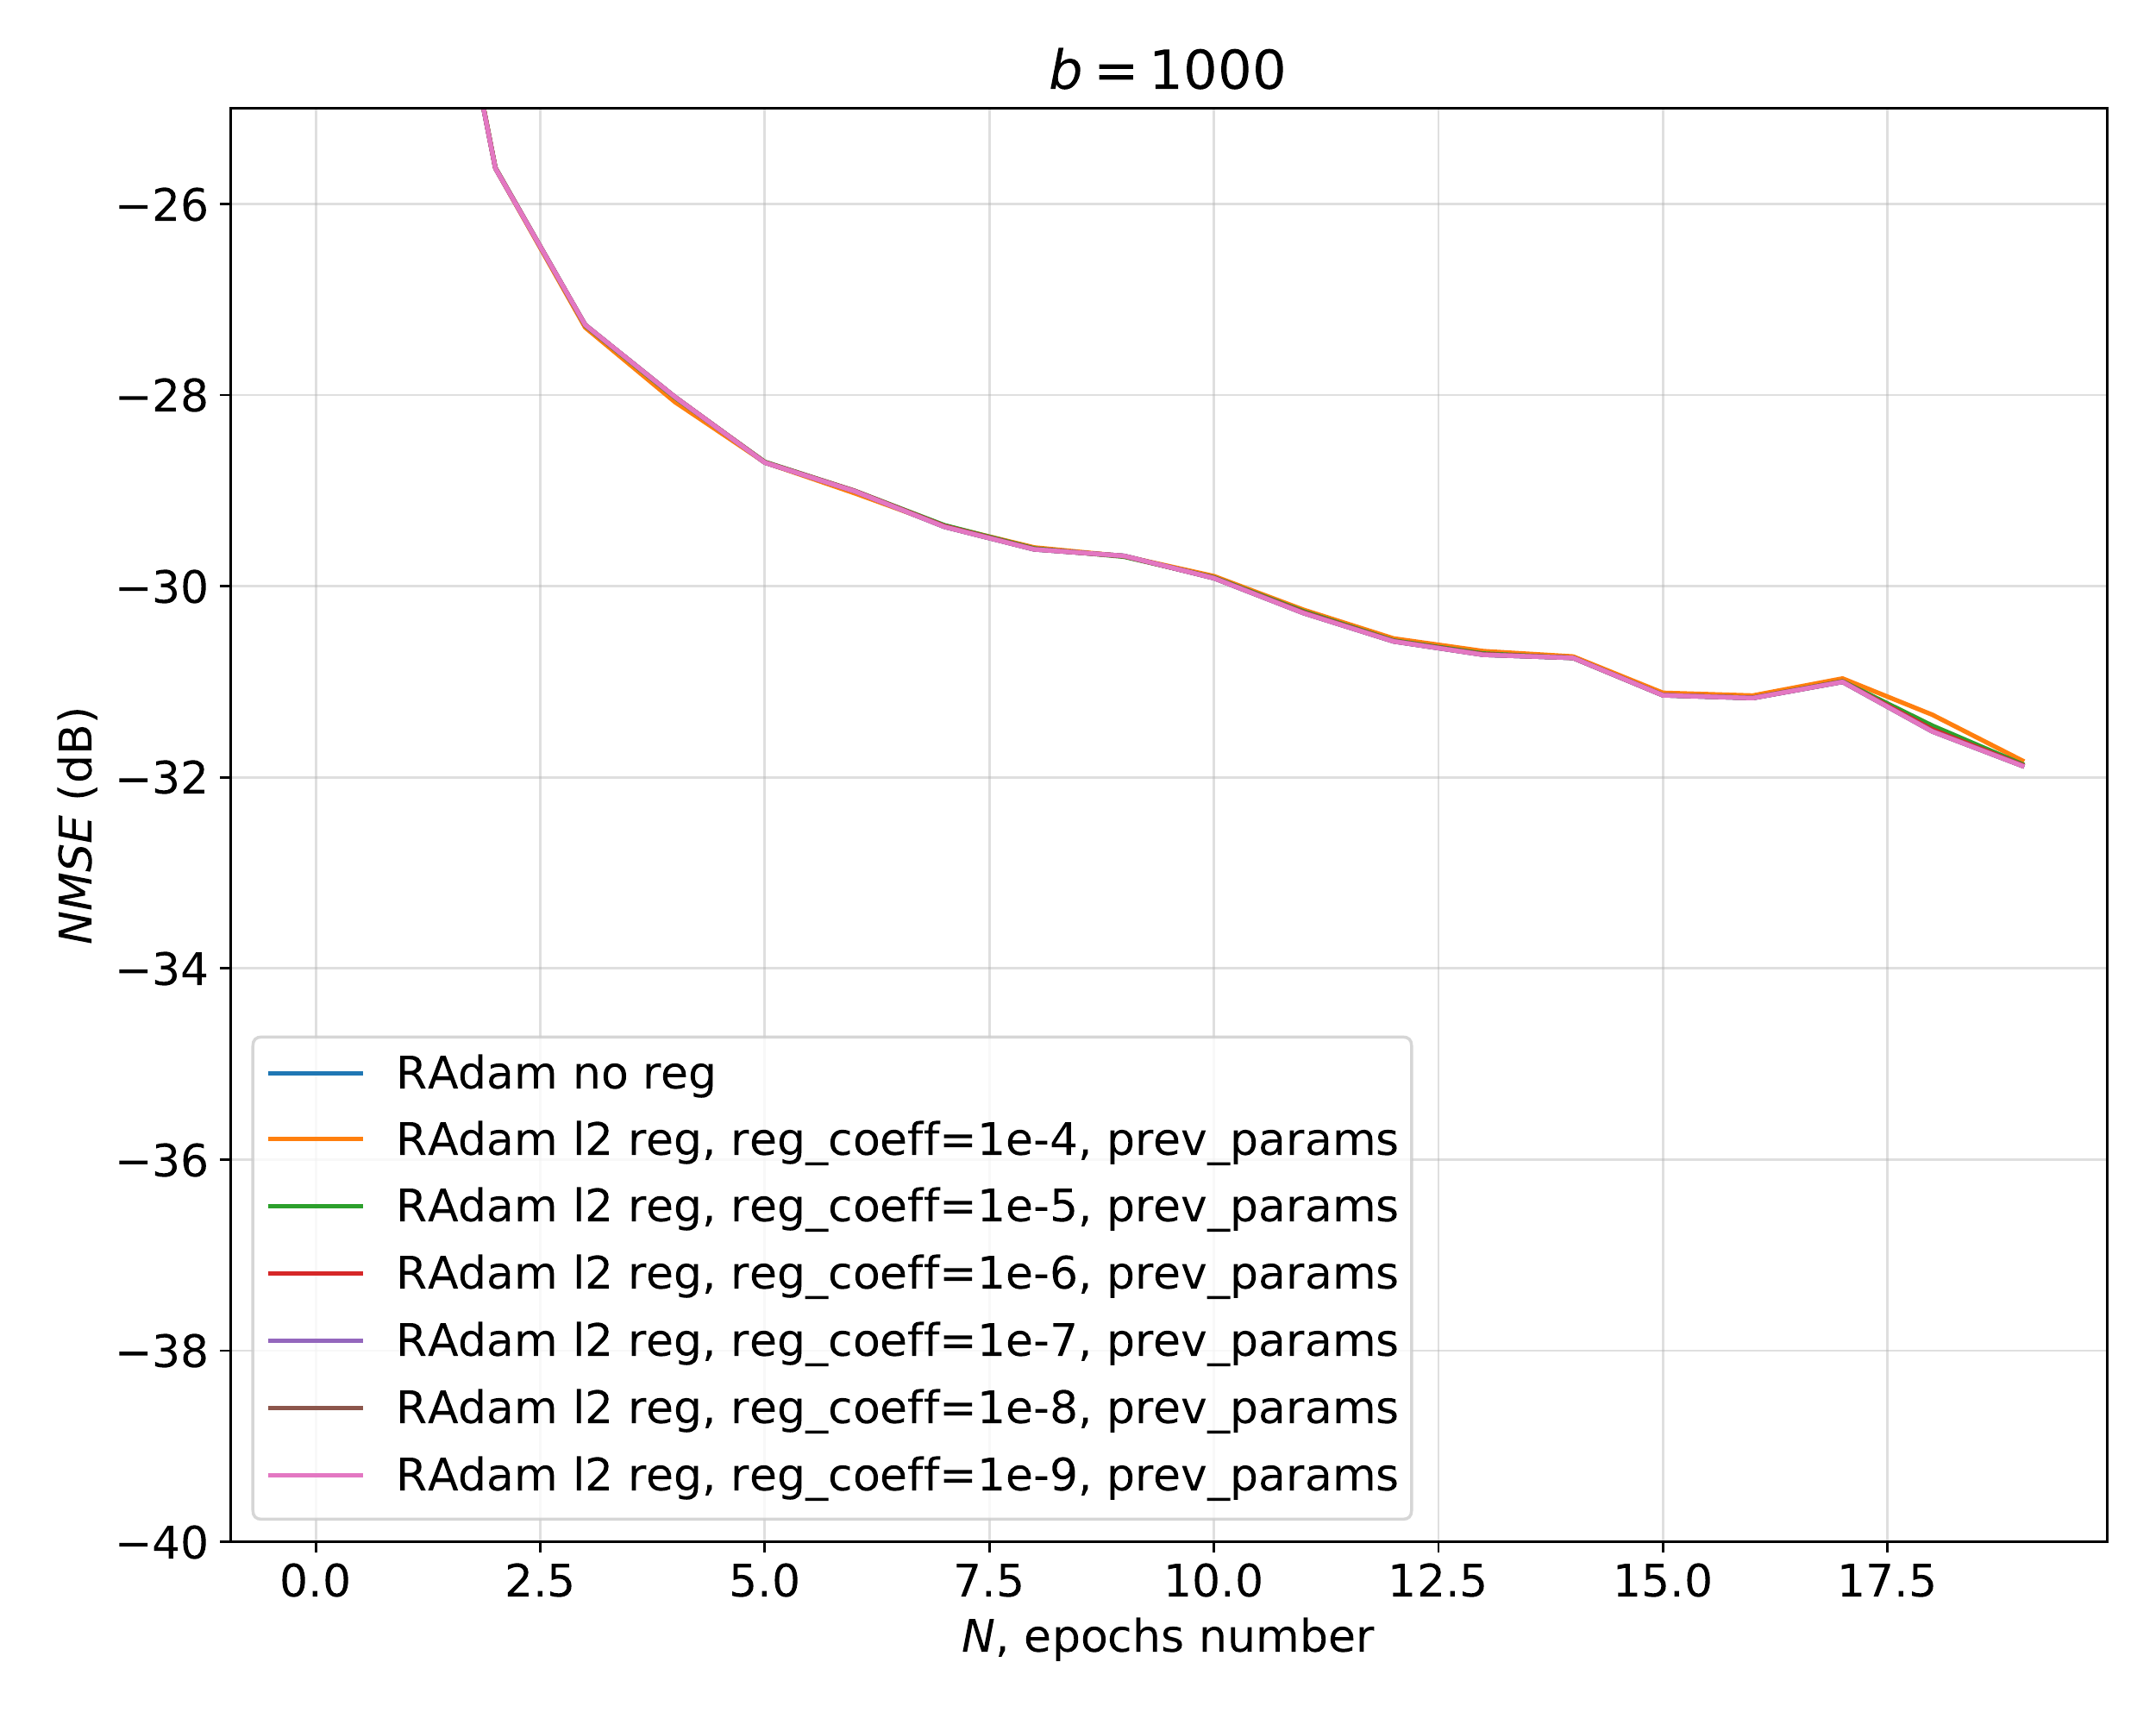}}}

\end{figure}

\begin{figure}[H]
    \centering
    \subfloat[Регуляризация для метода Adam]{{\includegraphics[width=0.45\textwidth]{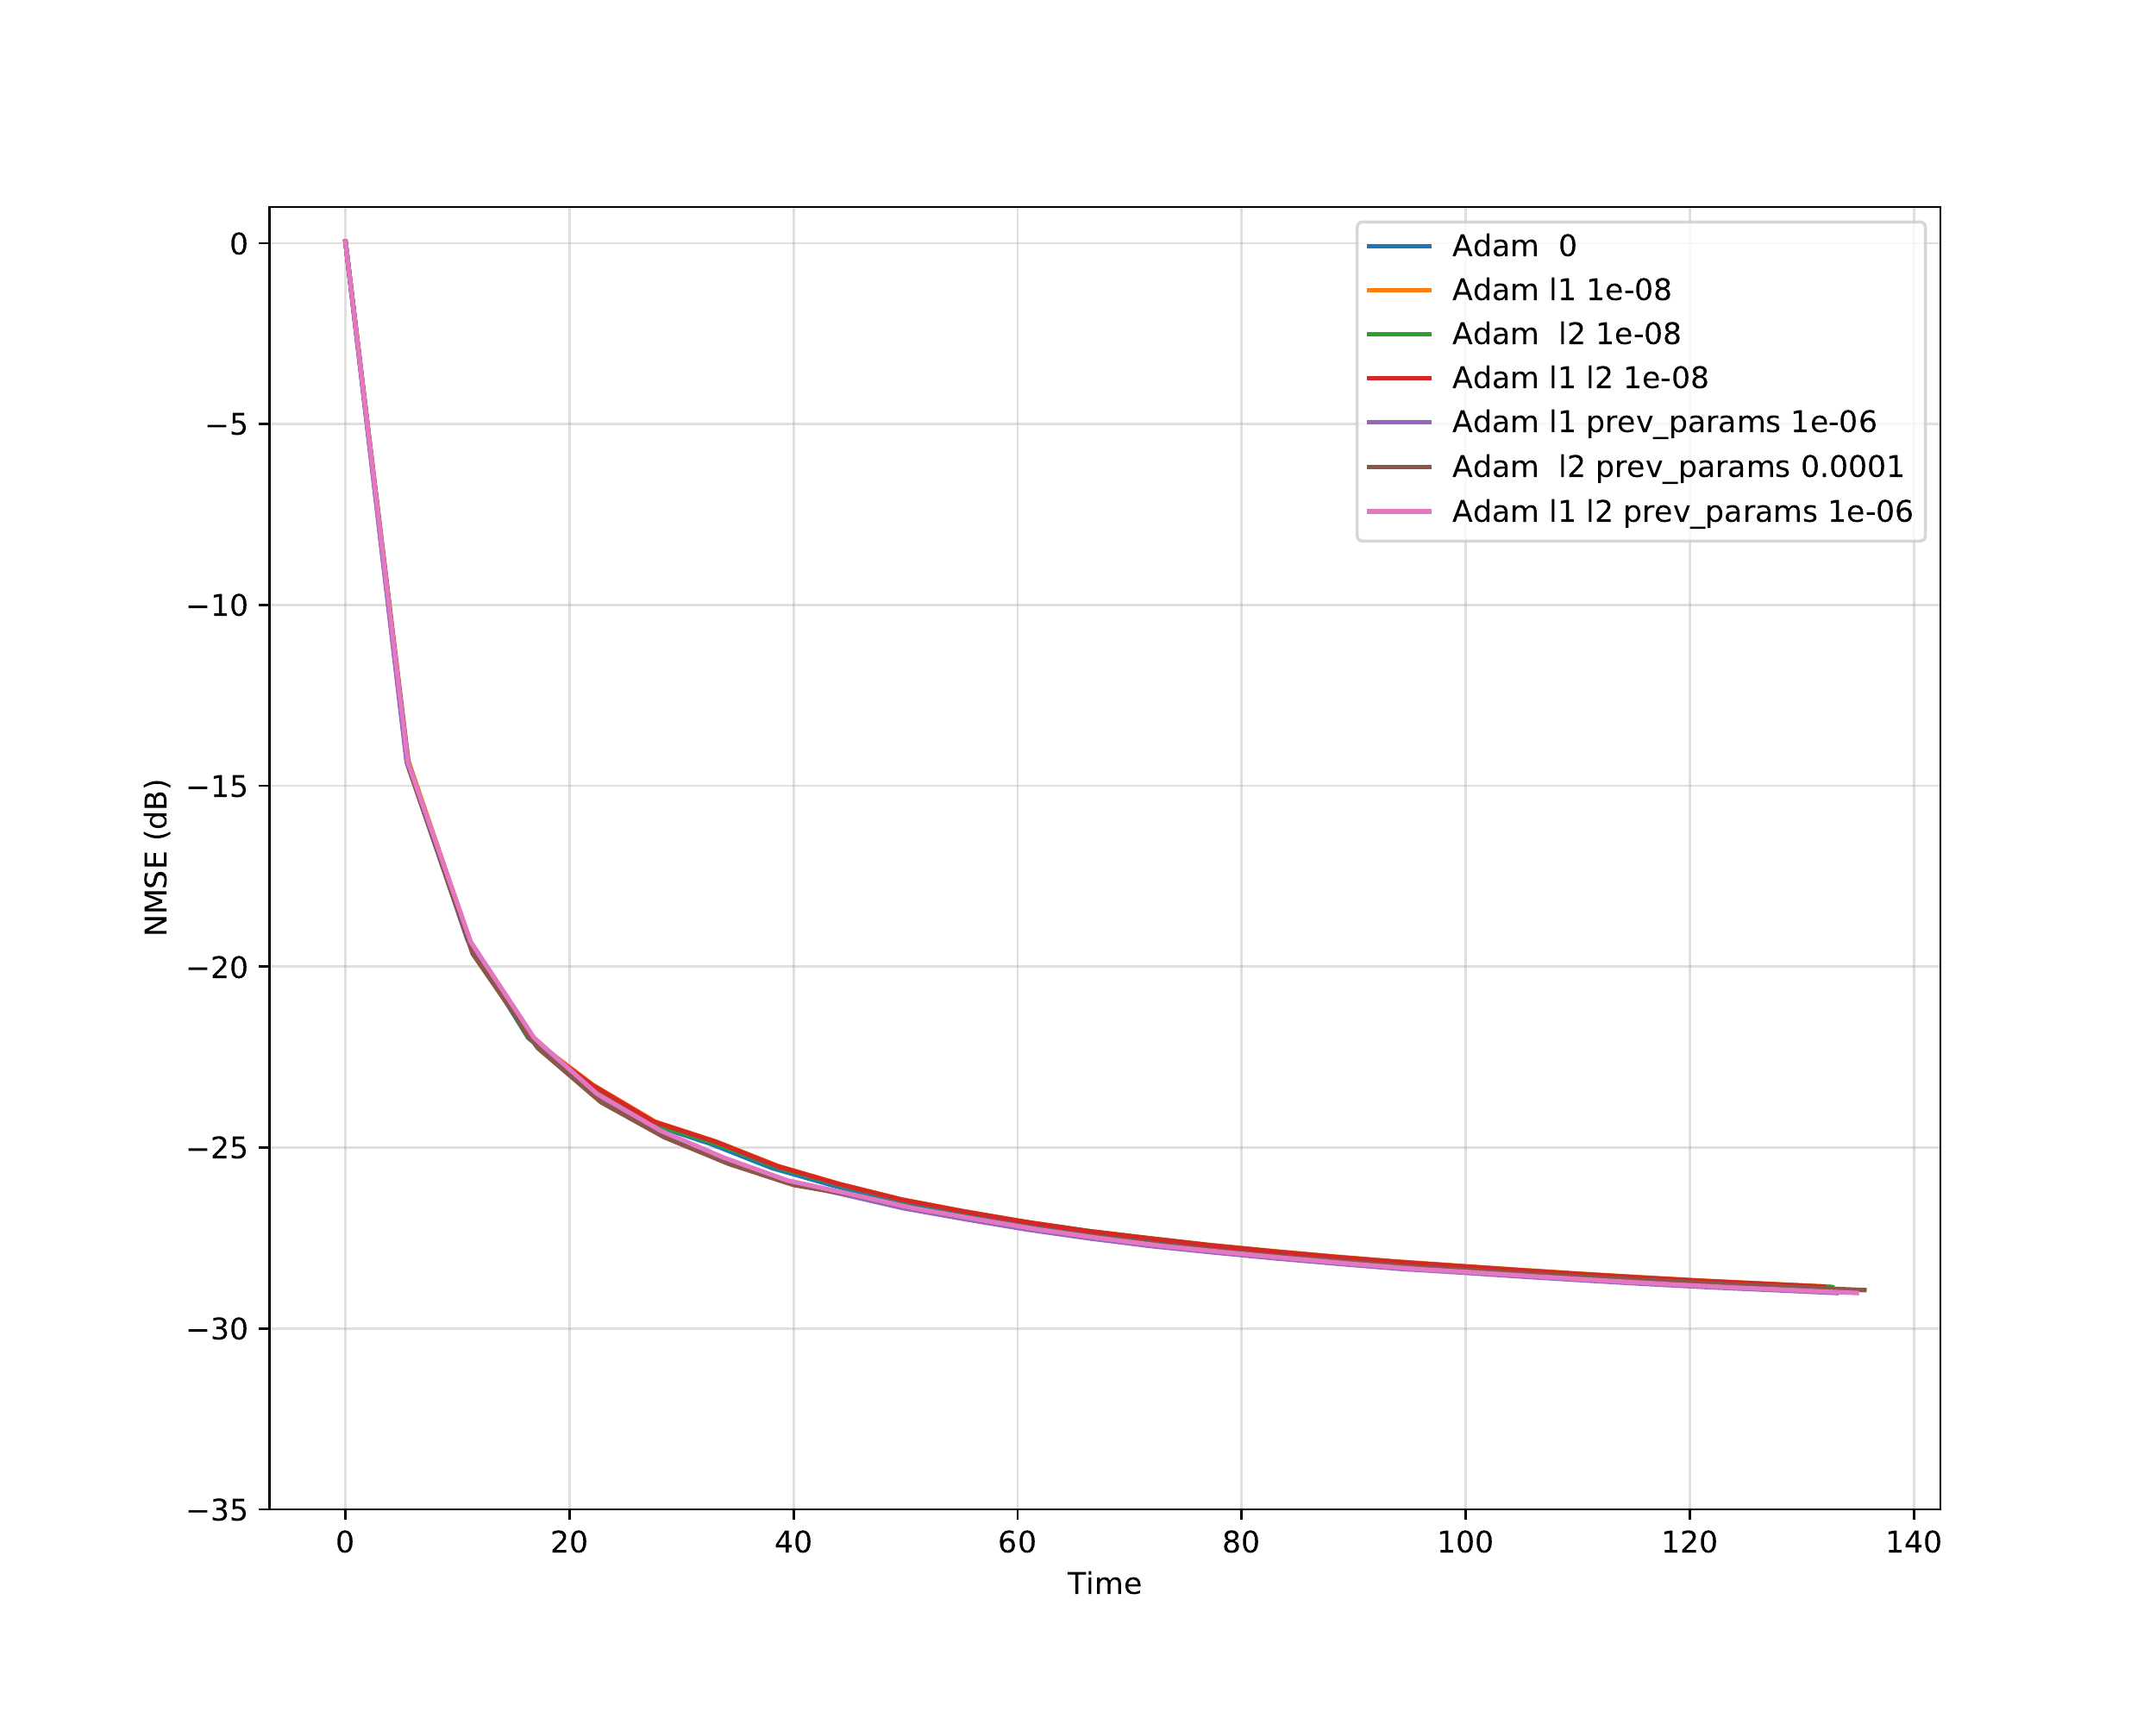}}}
    \subfloat[Циклический и статичный lr]{{\includegraphics[width=0.45\textwidth]{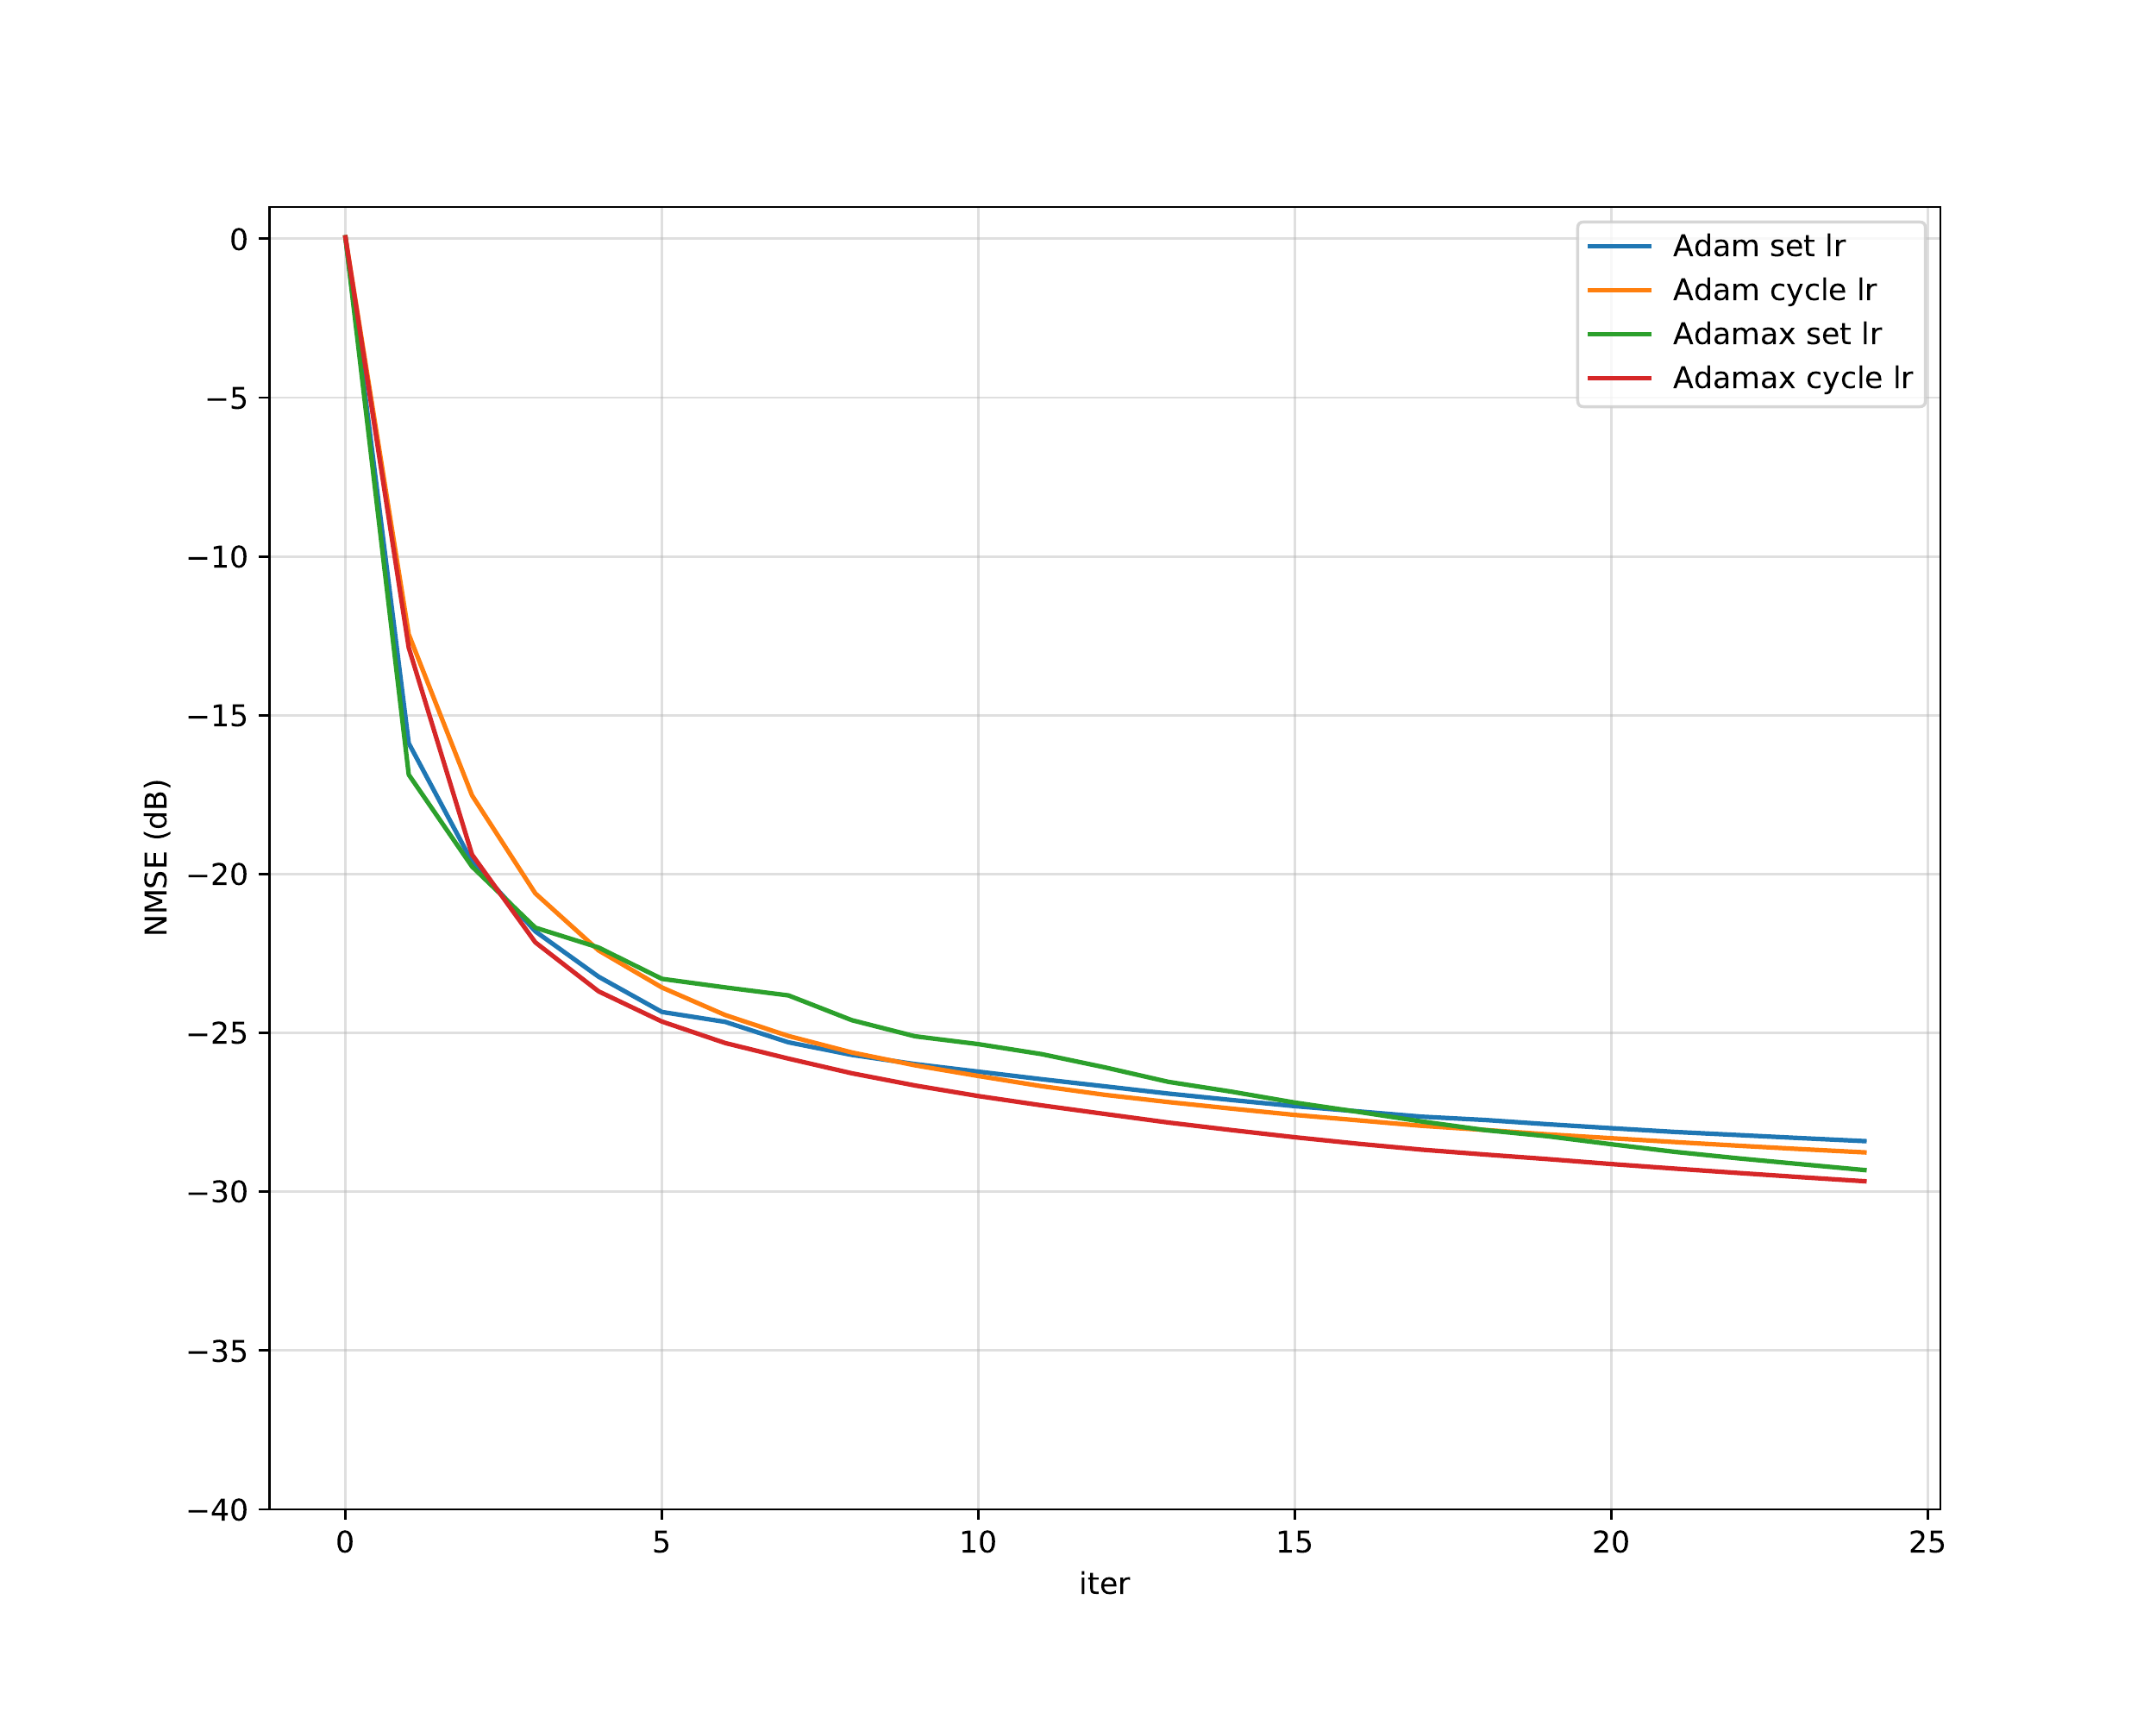}}}
    \caption{NMSE для различных методов в онлайне}
    \label{_reg}
\end{figure}
